# Supplementary material for: The impact of coarsening an exposure on partial identifiability in instrumental variable settings
Source: arXiv:2401.17735 ancillary file (2024-01-31)
Supplement: Supplementary file 1 [file supplementary-material.pdf]

# Supplementary Materials for: "The impact of coarsening an exposure on partial identifiability in instrumental variable settings"

Erin E. Gabriel[1*]
Michael C. Sachs[1]
Arvid Sjölander[2]
1: Section of Biostatistics, Department of Public Health, University of Copenhagen, Denmark
2: Department of Medical Epidemiology and Biostatistics, Karolinska Institutet, Stockholm, Sweden
corresponding author: erin.gabriel@sund.ku.dk

January 31, 2024

## S1 Novel Bounds

### S1.1 Result 1

Bounds on $\theta_{x'x}$ in terms of $p_{xy\cdot z} = p(X = x, Y = y|Z = z)$ where $X$ has 2 well-defining levels, and $Z$ has 2 levels in our notation, as given in Balke and Pearl [1997] and Balke [1995]:

$$\geq \max \left\{ \begin{array}{l} -1 + p_{x0\cdot 0} + p_{x'1\cdot 0}, \\ -1 + p_{x0\cdot 1} + p_{x'1\cdot 1}, \\ -2 + 2p_{x0\cdot 0} + p_{x1\cdot 1} + p_{x'1\cdot 0} + p_{x'1\cdot 1}, \\ -2 + p_{x0\cdot 0} + p_{x0\cdot 1} + p_{x'0\cdot 0} + 2p_{x'1\cdot 1}, \\ -1 + p_{x0\cdot 0} + p_{x'1\cdot 1}, \\ -2 + 2p_{x0\cdot 1} + p_{x1\cdot 0} + p_{x'1\cdot 0} + p_{x'1\cdot 1}, \\ -2 + p_{x0\cdot 0} + p_{x0\cdot 1} + p_{x'0\cdot 1} + 2p_{x'1\cdot 0}, \\ -1 + p_{x0\cdot 1} + p_{x'1\cdot 0} \end{array} \right\}$$

*EEG is partially supported Novo Nordisk foundation NNF22OC0076595

$$\leq \min \left\{ \begin{array}{l} 1 - p_{x'0\cdot 0} - p_{x1\cdot 0}, \\ 1 - p_{x'0\cdot 1} - p_{x1\cdot 1}, \\ 2 - p_{x0\cdot 1} - p_{x'0\cdot 0} - p_{x'0\cdot 1} - 2p_{x1\cdot 0}, \\ 2 - 2p_{x'0\cdot 1} - p_{x1\cdot 0} - p_{x1\cdot 1} - p_{x'1\cdot 0}, \\ 1 - p_{x'0\cdot 1} - p_{x1\cdot 0}, \\ 2 - 2p_{x'0\cdot 0} - p_{x1\cdot 0} - p_{x1\cdot 1} - p_{x'1\cdot 1}, \\ 2 - p_{x0\cdot 0} - p_{x'0\cdot 0} - p_{x'0\cdot 1} - 2p_{x1\cdot 1}, \\ 1 - p_{x'0\cdot 0} - p_{x1\cdot 1} \end{array} \right\}$$

## S1.2 Result 3

Bounds on $\theta_{x'x}$ in terms of $p_{xy\cdot z} = p(X = x, Y = y|Z = z)$ where $Z$ has 3 levels and either $X$ has 2 well-defining levels, or there is a third ill-defining level of $X$, or there is a third well-defining level of $X$ for which there is a direct effect of $Z$ on $Y$:

$$\begin{aligned}
\geq \max\{ & -p_{x0\cdot 0} - p_{x'0\cdot 0} + p_{x0\cdot 1} - p_{x1\cdot 0}, \\
& -p_{x0\cdot 0} - p_{x'0\cdot 0} + p_{x0\cdot 1} - p_{x'0\cdot 1} - p_{x1\cdot 1}, \\
& -p_{x0\cdot 0} - 2p_{x'0\cdot 0} + p_{x0\cdot 1} + p_{x'0\cdot 1} - 2p_{x1\cdot 0}, \\
& p_{x0\cdot 1} + p_{x'0\cdot 1} - p_{x0\cdot 2} - 2p_{x'0\cdot 2} - 2p_{x1\cdot 2}, \\
& p_{x0\cdot 1} - p_{x'0\cdot 1} - p_{x0\cdot 2} - p_{x'0\cdot 2} - p_{x1\cdot 1}, \\
& p_{x0\cdot 1} - p_{x0\cdot 2} - p_{x'0\cdot 2} - p_{x1\cdot 2}, \\
& -p_{x0\cdot 0} - p_{x'0\cdot 0} + p_{x0\cdot 1} - p_{x'0\cdot 2} - p_{x1\cdot 2}, \\
& -p_{x0\cdot 0} - p_{x'0\cdot 0} + p_{x0\cdot 1} + p_{x'0\cdot 1} - p_{x'0\cdot 2} - p_{x1\cdot 0} - p_{x1\cdot 2}, \\
& -p_{x0\cdot 0} - p_{x'0\cdot 0} + p_{x0\cdot 1} + p_{x'0\cdot 1} - 2p_{x'0\cdot 2} - 2p_{x1\cdot 2}, \\
& -2p_{x'0\cdot 0} + p_{x0\cdot 1} + p_{x'0\cdot 1} - p_{x0\cdot 2} - p_{x'0\cdot 2} - 2p_{x1\cdot 0}, \\
& -p_{x'0\cdot 0} + p_{x0\cdot 1} + p_{x'0\cdot 1} - p_{x0\cdot 2} - p_{x'0\cdot 2} - p_{x1\cdot 0} - p_{x1\cdot 2}, \\
& -p_{x'0\cdot 0} + p_{x0\cdot 1} - p_{x0\cdot 2} - p_{x'0\cdot 2} - p_{x1\cdot 0}, \\
& p_{x0\cdot 0} - p_{x0\cdot 1} - p_{x'0\cdot 1} - p_{x1\cdot 1}, \\
& p_{x0\cdot 0} - p_{x'0\cdot 0} - p_{x0\cdot 1} - p_{x'0\cdot 1} - p_{x1\cdot 0}, \\
& p_{x0\cdot 0} + p_{x'0\cdot 0} - p_{x0\cdot 1} - 2p_{x'0\cdot 1} - 2p_{x1\cdot 1}, \\
& p_{x0\cdot 0} + p_{x'0\cdot 0} - p_{x0\cdot 2} - 2p_{x'0\cdot 2} - 2p_{x1\cdot 2}, \\
& p_{x0\cdot 0} - p_{x'0\cdot 0} - p_{x0\cdot 2} - p_{x'0\cdot 2} - p_{x1\cdot 0}, \\
& p_{x0\cdot 0} - p_{x0\cdot 2} - p_{x'0\cdot 2} - p_{x1\cdot 2}, \\
& p_{x0\cdot 0} - p_{x0\cdot 1} - p_{x'0\cdot 1} - p_{x'0\cdot 2} - p_{x1\cdot 2}, \\
& p_{x0\cdot 0} + p_{x'0\cdot 0} - p_{x0\cdot 1} - p_{x'0\cdot 1} - p_{x'0\cdot 2} - p_{x1\cdot 1} - p_{x1\cdot 2}, \\
& p_{x0\cdot 0} + p_{x'0\cdot 0} - p_{x0\cdot 1} - p_{x'0\cdot 1} - 2p_{x'0\cdot 2} - 2p_{x1\cdot 2}, \\
& p_{x0\cdot 0} + p_{x'0\cdot 0} - 2p_{x'0\cdot 1} - p_{x0\cdot 2} - p_{x'0\cdot 2} - 2p_{x1\cdot 1}, \\
& p_{x0\cdot 0} + p_{x'0\cdot 0} - p_{x'0\cdot 1} - p_{x0\cdot 2} - p_{x'0\cdot 2} - p_{x1\cdot 1} - p_{x1\cdot 2},
\end{aligned}$$

$$p_{x0\cdot0} - p_{x'0\cdot1} - p_{x0\cdot2} - p_{x'0\cdot2} - p_{x1\cdot1},$$
$$- p_{x'0\cdot0} - p_{x1\cdot0},$$
$$- p_{x'0\cdot1} - p_{x1\cdot1},$$
$$- p_{x'0\cdot2} - p_{x1\cdot2},$$
$$- p_{x'0\cdot0} - p_{x0\cdot1} - p_{x'0\cdot1} + p_{x0\cdot2} - p_{x1\cdot0},$$
$$- p_{x'0\cdot0} - p_{x0\cdot1} - p_{x'0\cdot1} + p_{x0\cdot2} + p_{x'0\cdot2} - p_{x1\cdot0} - p_{x1\cdot1},$$
$$- 2p_{x'0\cdot0} - p_{x0\cdot1} - p_{x'0\cdot1} + p_{x0\cdot2} + p_{x'0\cdot2} - 2p_{x1\cdot0},$$
$$- p_{x0\cdot0} - p_{x'0\cdot0} - 2p_{x'0\cdot1} + p_{x0\cdot2} + p_{x'0\cdot2} - 2p_{x1\cdot1},$$
$$- p_{x0\cdot0} - p_{x'0\cdot0} - p_{x'0\cdot1} + p_{x0\cdot2} - p_{x1\cdot1},$$
$$- p_{x0\cdot0} - p_{x'0\cdot0} - p_{x'0\cdot1} + p_{x0\cdot2} + p_{x'0\cdot2} - p_{x1\cdot0} - p_{x1\cdot1},$$
$$- p_{x0\cdot0} - p_{x'0\cdot0} + p_{x0\cdot2} - p_{x1\cdot0},$$
$$- p_{x0\cdot0} - p_{x'0\cdot0} + p_{x0\cdot2} - p_{x'0\cdot2} - p_{x1\cdot2},$$
$$- p_{x0\cdot0} - 2p_{x'0\cdot0} + p_{x0\cdot2} + p_{x'0\cdot2} - 2p_{x1\cdot0},$$
$$- p_{x0\cdot1} - p_{x'0\cdot1} + p_{x0\cdot2} - p_{x1\cdot1},$$
$$- p_{x0\cdot1} - p_{x'0\cdot1} + p_{x0\cdot2} - p_{x'0\cdot2} - p_{x1\cdot2},$$
$$- p_{x0\cdot1} - 2p_{x'0\cdot1} + p_{x0\cdot2} + p_{x'0\cdot2} - 2p_{x1\cdot1}\}$$

$$\leq \max\{1 - p_{x'0\cdot0} - p_{x1\cdot1},$$
$$2 - p_{x0\cdot0} - p_{x'0\cdot0} - p_{x'0\cdot1} - 2p_{x1\cdot1},$$
$$1 - 2p_{x'0\cdot0} + p_{x0\cdot1} + p_{x'0\cdot1} - p_{x1\cdot0},$$
$$2 - p_{x'0\cdot1} - p_{x0\cdot2} - p_{x'0\cdot2} - 2p_{x1\cdot1},$$
$$1 + p_{x0\cdot1} + p_{x'0\cdot1} - 2p_{x'0\cdot2} - p_{x1\cdot2},$$
$$1 - p_{x'0\cdot2} - p_{x1\cdot1},$$
$$2 - p_{x0\cdot0} - p_{x'0\cdot0} - p_{x'0\cdot2} - p_{x1\cdot1} - p_{x1\cdot2},$$
$$1 - p_{x'0\cdot0} + p_{x0\cdot1} + p_{x'0\cdot1} - p_{x'0\cdot2} - p_{x1\cdot2},$$
$$2 - p_{x0\cdot0} - p_{x'0\cdot0} + p_{x0\cdot1} + p_{x'0\cdot1} - 2p_{x'0\cdot2} - 2p_{x1\cdot2},$$
$$2 - 2p_{x'0\cdot0} + p_{x0\cdot1} + p_{x'0\cdot1} - p_{x0\cdot2} - p_{x'0\cdot2} - 2p_{x1\cdot0},$$
$$1 - p_{x'0\cdot0} + p_{x0\cdot1} + p_{x'0\cdot1} - p_{x'0\cdot2} - p_{x1\cdot0},$$
$$2 - p_{x'0\cdot0} - p_{x0\cdot2} - p_{x'0\cdot2} - p_{x1\cdot0} - p_{x1\cdot1},$$
$$1 - p_{x'0\cdot1} - p_{x1\cdot0},$$
$$1 + p_{x0\cdot0} + p_{x'0\cdot0} - 2p_{x'0\cdot1} - p_{x1\cdot1},$$
$$2 - p_{x'0\cdot0} - p_{x0\cdot1} - p_{x'0\cdot1} - 2p_{x1\cdot0},$$
$$2 - p_{x'0\cdot0} - p_{x0\cdot2} - p_{x'0\cdot2} - 2p_{x1\cdot0},$$
$$1 + p_{x0\cdot0} + p_{x'0\cdot0} - 2p_{x'0\cdot2} - p_{x1\cdot2},$$
$$1 - p_{x'0\cdot2} - p_{x1\cdot0},$$
$$2 - p_{x0\cdot1} - p_{x'0\cdot1} - p_{x'0\cdot2} - p_{x1\cdot0} - p_{x1\cdot2},$$
$$1 + p_{x0\cdot0} + p_{x'0\cdot0} - p_{x'0\cdot1} - p_{x'0\cdot2} - p_{x1\cdot2},$$

$$
\begin{aligned}
&2 + p_{x0\cdot 0} + p_{x'0\cdot 0} - p_{x0\cdot 1} - p_{x'0\cdot 1} - 2p_{x'0\cdot 2} - 2p_{x1\cdot 2},\\
&2 + p_{x0\cdot 0} + p_{x'0\cdot 0} - 2p_{x'0\cdot 1} - p_{x0\cdot 2} - p_{x'0\cdot 2} - 2p_{x1\cdot 1},\\
&1 + p_{x0\cdot 0} + p_{x'0\cdot 0} - p_{x'0\cdot 1} - p_{x'0\cdot 2} - p_{x1\cdot 1},\\
&2 - p_{x'0\cdot 1} - p_{x0\cdot 2} - p_{x'0\cdot 2} - p_{x1\cdot 0} - p_{x1\cdot 1},\\
&1 - p_{x'0\cdot 2} - p_{x1\cdot 2},\\
&1 - p_{x'0\cdot 0} - p_{x1\cdot 0},\\
&1 - p_{x'0\cdot 1} - p_{x1\cdot 1},\\
&2 - p_{x'0\cdot 0} - p_{x0\cdot 1} - p_{x'0\cdot 1} - p_{x1\cdot 0} - p_{x1\cdot 2},\\
&1 - p_{x'0\cdot 0} - p_{x'0\cdot 1} + p_{x0\cdot 2} + p_{x'0\cdot 2} - p_{x1\cdot 0},\\
&2 - 2p_{x'0\cdot 0} - p_{x0\cdot 1} - p_{x'0\cdot 1} + p_{x0\cdot 2} + p_{x'0\cdot 2} - 2p_{x1\cdot 0},\\
&2 - p_{x0\cdot 0} - p_{x'0\cdot 0} - 2p_{x'0\cdot 1} + p_{x0\cdot 2} + p_{x'0\cdot 2} - 2p_{x1\cdot 1},\\
&2 - p_{x0\cdot 0} - p_{x'0\cdot 0} - p_{x'0\cdot 1} - p_{x1\cdot 1} - p_{x1\cdot 2},\\
&1 - p_{x'0\cdot 0} - p_{x'0\cdot 1} + p_{x0\cdot 2} + p_{x'0\cdot 2} - p_{x1\cdot 1},\\
&1 - p_{x'0\cdot 0} - p_{x1\cdot 2},\\
&2 - p_{x0\cdot 0} - p_{x'0\cdot 0} - p_{x'0\cdot 2} - 2p_{x1\cdot 2},\\
&1 - 2p_{x'0\cdot 0} + p_{x0\cdot 2} + p_{x'0\cdot 2} - p_{x1\cdot 0},\\
&1 - p_{x'0\cdot 1} - p_{x1\cdot 2},\\
&2 - p_{x0\cdot 1} - p_{x'0\cdot 1} - p_{x'0\cdot 2} - 2p_{x1\cdot 2},\\
&1 - 2p_{x'0\cdot 1} + p_{x0\cdot 2} + p_{x'0\cdot 2} - p_{x1\cdot 1}\}
\end{aligned}
$$

## S1.3 Result 4

Bounds on $\theta_{x'x}$ in terms of $p_{xy\cdot z} = p(X = x, Y = y|Z = z)$ where $Z$ has 3 levels and either $X$ has 3 well-defining levels, or there is a fourth ill-defining level of $X$, or there is a fourth well-defining level of $X$ for which there is a direct effect of $Z$ on $Y$:

$$
\begin{aligned}
\geq \max\{ &-2 + 2p_{x0\cdot 2} + p_{x1\cdot 0} + p_{x'1\cdot 0} + p_{x'1\cdot 2},\\
&-2 + p_{x0\cdot 0} + p_{x0\cdot 2} + p_{x'0\cdot 2} + 2p_{x'1\cdot 0},\\
&-1 + p_{x0\cdot 2} + p_{x'1\cdot 0},\\
&-2 + p_{x0\cdot 0} + p_{x0\cdot 2} - p_{x'0\cdot 1} + p_{x'0\cdot 2} + p_{x''0\cdot 0} - p_{x''0\cdot 1} - p_{x1\cdot 1} + 2p_{x'1\cdot 0},\\
&-2 + 2p_{x0\cdot 2} - p_{x'0\cdot 1} - p_{x''0\cdot 1} + p_{x''0\cdot 2} + p_{x1\cdot 0} - p_{x1\cdot 1} + p_{x'1\cdot 0} + p_{x'1\cdot 2},\\
&-2 - p_{x0\cdot 1} + 2p_{x0\cdot 2} - p_{x'0\cdot 1} + p_{x''0\cdot 0} - p_{x''0\cdot 1} + p_{x1\cdot 0} + p_{x'1\cdot 0} + p_{x'1\cdot 2},\\
&-2 + p_{x0\cdot 0} - p_{x0\cdot 1} + p_{x0\cdot 2} - 2p_{x'0\cdot 1} + p_{x'0\cdot 2} + 2p_{x''0\cdot 0} - 2p_{x''0\cdot 1} - 2p_{x1\cdot 1} + 2p_{x'1\cdot 0},\\
&-2 - p_{x0\cdot 1} + 2p_{x0\cdot 2} - p_{x'0\cdot 1} + p_{x''0\cdot 0} - p_{x''0\cdot 1} + p_{x''0\cdot 2} + p_{x1\cdot 0} - p_{x1\cdot 1} + p_{x'1\cdot 0} + p_{x'1\cdot 2},\\
&-1 - p_{x0\cdot 1} + p_{x0\cdot 2} - p_{x'0\cdot 1} - p_{x'0\cdot 2} + p_{x''0\cdot 0} - p_{x''0\cdot 1} - p_{x''0\cdot 2} - p_{x1\cdot 2} + p_{x'1\cdot 0},\\
&-1 - p_{x0\cdot 1} + p_{x0\cdot 2} - p_{x'0\cdot 1} + p_{x''0\cdot 0} - p_{x''0\cdot 1} - p_{x1\cdot 1} + p_{x'1\cdot 0},\\
&-2 + 2p_{x0\cdot 2} - 2p_{x'0\cdot 1} - 2p_{x''0\cdot 1} + 2p_{x''0\cdot 2} + p_{x1\cdot 0} - 2p_{x1\cdot 1} + p_{x'1\cdot 0} - p_{x'1\cdot 1} + p_{x'1\cdot 2},\\
&-2 + p_{x0\cdot 0} + p_{x0\cdot 2} + p_{x'0\cdot 2} - p_{x''0\cdot 1} + p_{x''0\cdot 2} - p_{x1\cdot 1} + 2p_{x'1\cdot 0} - p_{x'1\cdot 1},
\end{aligned}
$$

$- 2 + p_{x0\cdot 0} + p_{x0\cdot 2} - p_{x'0\cdot 1} + p_{x'0\cdot 2} + p_{x''0\cdot 0} - p_{x''0\cdot 1} + p_{x''0\cdot 2} - p_{x1\cdot 1} + 2p_{x'1\cdot 0} - p_{x'1\cdot 1},$

$- 1 + p_{x0\cdot 2} - p_{x'0\cdot 0} - p_{x''0\cdot 0} - p_{x''0\cdot 1} + p_{x''0\cdot 2} - p_{x1\cdot 0} - p_{x1\cdot 1} + p_{x'1\cdot 0} - p_{x'1\cdot 1},$

$- 1 + p_{x0\cdot 2} - p_{x'0\cdot 1} - p_{x''0\cdot 1} + p_{x''0\cdot 2} - p_{x1\cdot 1} + p_{x'1\cdot 0} - p_{x'1\cdot 1},$

$- 1 - p_{x0\cdot 1} + p_{x0\cdot 2} - 2p_{x'0\cdot 1} + p_{x''0\cdot 0} - 2p_{x''0\cdot 1} + p_{x''0\cdot 2} - 2p_{x1\cdot 1} + p_{x'1\cdot 0} - p_{x'1\cdot 1},$

$- 2 + p_{x0\cdot 0} - p_{x0\cdot 1} + p_{x0\cdot 2} - 2p_{x'0\cdot 1} + p_{x'0\cdot 2} + 2p_{x''0\cdot 0} - 2p_{x''0\cdot 1} + p_{x''0\cdot 2} - 2p_{x1\cdot 1} + 2p_{x'1\cdot 0} - p_{x'1\cdot 1},$

$- 2 - p_{x0\cdot 1} + 2p_{x0\cdot 2} - 2p_{x'0\cdot 1} + p_{x''0\cdot 0} - 2p_{x''0\cdot 1} + 2p_{x''0\cdot 2} + p_{x1\cdot 0} - 2p_{x1\cdot 1} + p_{x'1\cdot 0} - p_{x'1\cdot 1} + p_{x'1\cdot 2},$

$- 1 + p_{x0\cdot 0} - p_{x0\cdot 1} - p_{x'0\cdot 1} - p_{x'0\cdot 2} + 2p_{x''0\cdot 0} - p_{x''0\cdot 1} - p_{x''0\cdot 2} - p_{x1\cdot 1} - p_{x1\cdot 2} + p_{x'1\cdot 0} - p_{x'1\cdot 2},$

$- 2 + 2p_{x0\cdot 0} - 2p_{x'0\cdot 2} + 2p_{x''0\cdot 0} - 2p_{x''0\cdot 2} + p_{x1\cdot 1} - 2p_{x1\cdot 2} + p_{x'1\cdot 0} + p_{x'1\cdot 1} - p_{x'1\cdot 2},$

$- 2 + p_{x0\cdot 0} + p_{x0\cdot 1} + p_{x'0\cdot 0} + p_{x''0\cdot 0} - p_{x''0\cdot 2} - p_{x1\cdot 2} + 2p_{x'1\cdot 1} - p_{x'1\cdot 2},$

$- 2 + p_{x0\cdot 0} + p_{x0\cdot 1} + p_{x'0\cdot 0} - p_{x'0\cdot 2} + p_{x''0\cdot 0} + p_{x''0\cdot 1} - p_{x''0\cdot 2} - p_{x1\cdot 2} + 2p_{x'1\cdot 1} - p_{x'1\cdot 2},$

$- 1 + p_{x0\cdot 0} - p_{x'0\cdot 2} + p_{x''0\cdot 0} - p_{x''0\cdot 2} - p_{x1\cdot 2} + p_{x'1\cdot 1} - p_{x'1\cdot 2},$

$- 1 + p_{x0\cdot 0} - p_{x'0\cdot 1} + p_{x''0\cdot 0} - p_{x''0\cdot 1} - p_{x''0\cdot 2} - p_{x1\cdot 1} - p_{x1\cdot 2} + p_{x'1\cdot 1} - p_{x'1\cdot 2},$

$- 1 + p_{x0\cdot 0} - p_{x0\cdot 1} - 2p_{x'0\cdot 1} + 2p_{x''0\cdot 0} - 2p_{x''0\cdot 1} - p_{x''0\cdot 2} - 2p_{x1\cdot 1} - p_{x1\cdot 2} + p_{x'1\cdot 0} - p_{x'1\cdot 2},$

$- 1 + p_{x0\cdot 0} - p_{x0\cdot 1} - p_{x'0\cdot 1} - 2p_{x'0\cdot 2} + 2p_{x''0\cdot 0} - p_{x''0\cdot 1} - 2p_{x''0\cdot 2} - 2p_{x1\cdot 2} + p_{x'1\cdot 0} - p_{x'1\cdot 2},$

$- 2 + 2p_{x0\cdot 1} + p_{x1\cdot 0} + p_{x'1\cdot 0} + p_{x'1\cdot 1},$

$- 2 + p_{x0\cdot 0} + p_{x0\cdot 1} + p_{x'0\cdot 1} + 2p_{x'1\cdot 0},$

$- 1 + p_{x0\cdot 1} + p_{x'1\cdot 0},$

$- 2 + p_{x0\cdot 0} + p_{x0\cdot 1} + p_{x'0\cdot 1} - p_{x'0\cdot 2} + p_{x''0\cdot 0} - p_{x''0\cdot 2} - p_{x1\cdot 2} + 2p_{x'1\cdot 0},$

$- 2 + 2p_{x0\cdot 1} - p_{x'0\cdot 2} + p_{x''0\cdot 1} - p_{x''0\cdot 2} + p_{x1\cdot 0} - p_{x1\cdot 2} + p_{x'1\cdot 0} + p_{x'1\cdot 1},$

$- 2 + 2p_{x0\cdot 1} - p_{x0\cdot 2} - p_{x'0\cdot 2} + p_{x''0\cdot 0} - p_{x''0\cdot 2} + p_{x1\cdot 0} + p_{x'1\cdot 0} + p_{x'1\cdot 1},$

$- 2 + p_{x0\cdot 0} + p_{x0\cdot 1} - p_{x0\cdot 2} + p_{x'0\cdot 1} - 2p_{x'0\cdot 2} + 2p_{x''0\cdot 0} - 2p_{x''0\cdot 2} - 2p_{x1\cdot 2} + 2p_{x'1\cdot 0},$

$- 2 + 2p_{x0\cdot 1} - p_{x0\cdot 2} - p_{x'0\cdot 2} + p_{x''0\cdot 0} + p_{x''0\cdot 1} - p_{x''0\cdot 2} + p_{x1\cdot 0} - p_{x1\cdot 2} + p_{x'1\cdot 0} + p_{x'1\cdot 1},$

$- 1 + p_{x0\cdot 1} - p_{x0\cdot 2} - p_{x'0\cdot 2} + p_{x''0\cdot 0} - p_{x''0\cdot 2} - p_{x1\cdot 2} + p_{x'1\cdot 0},$

$- 1 + p_{x0\cdot 1} - p_{x0\cdot 2} - p_{x'0\cdot 1} - p_{x'0\cdot 2} + p_{x''0\cdot 0} - p_{x''0\cdot 1} - p_{x''0\cdot 2} - p_{x1\cdot 1} + p_{x'1\cdot 0},$

$- 1 + p_{x0\cdot 1} - p_{x0\cdot 2} - 2p_{x'0\cdot 2} + p_{x''0\cdot 0} + p_{x''0\cdot 1} - 2p_{x''0\cdot 2} - 2p_{x1\cdot 2} + p_{x'1\cdot 0} - p_{x'1\cdot 2},$

$- 2 + p_{x0\cdot 0} + p_{x0\cdot 1} - p_{x0\cdot 2} + p_{x'0\cdot 1} - 2p_{x'0\cdot 2} + 2p_{x''0\cdot 0} + p_{x''0\cdot 1} - 2p_{x''0\cdot 2} - 2p_{x1\cdot 2} + 2p_{x'1\cdot 0} - p_{x'1\cdot 2},$

$- 2 + 2p_{x0\cdot 1} - p_{x0\cdot 2} - 2p_{x'0\cdot 2} + p_{x''0\cdot 0} + 2p_{x''0\cdot 1} - 2p_{x''0\cdot 2} + p_{x1\cdot 0} - 2p_{x1\cdot 2} + p_{x'1\cdot 0} + p_{x'1\cdot 1} - p_{x'1\cdot 2},$

$- 2 + 2p_{x0\cdot 0} - 2p_{x'0\cdot 1} + 2p_{x''0\cdot 0} - 2p_{x''0\cdot 1} - 2p_{x1\cdot 1} + p_{x1\cdot 2} + p_{x'1\cdot 0} - p_{x'1\cdot 1} + p_{x'1\cdot 2},$

$- 2 + p_{x0\cdot 0} + p_{x0\cdot 2} + p_{x'0\cdot 0} + p_{x''0\cdot 0} - p_{x''0\cdot 1} - p_{x1\cdot 1} - p_{x'1\cdot 1} + 2p_{x'1\cdot 2},$

$- 1 + p_{x0\cdot 0} - p_{x'0\cdot 2} + p_{x''0\cdot 0} - p_{x''0\cdot 1} - p_{x''0\cdot 2} - p_{x1\cdot 1} - p_{x1\cdot 2} - p_{x'1\cdot 1} + p_{x'1\cdot 2},$

$- 1 + p_{x0\cdot 0} - p_{x'0\cdot 1} + p_{x''0\cdot 0} - p_{x''0\cdot 1} - p_{x1\cdot 1} - p_{x'1\cdot 1} + p_{x'1\cdot 2},$

$- 2 + p_{x0\cdot 0} + p_{x0\cdot 2} + p_{x'0\cdot 0} - p_{x'0\cdot 1} + p_{x''0\cdot 0} - p_{x''0\cdot 1} + p_{x''0\cdot 2} - p_{x1\cdot 1} - p_{x'1\cdot 1} + 2p_{x'1\cdot 2},$

$- 1 + p_{x0\cdot 0} - p_{x0\cdot 2} - p_{x'0\cdot 1} - p_{x'0\cdot 2} + 2p_{x''0\cdot 0} - p_{x''0\cdot 1} - p_{x''0\cdot 2} - p_{x1\cdot 1} - p_{x1\cdot 2} + p_{x'1\cdot 0} - p_{x'1\cdot 1},$

$- 1 + p_{x0\cdot 0} - p_{x0\cdot 2} - 2p_{x'0\cdot 1} - p_{x'0\cdot 2} + 2p_{x''0\cdot 0} - 2p_{x''0\cdot 1} - p_{x''0\cdot 2} - 2p_{x1\cdot 1} + p_{x'1\cdot 0} - p_{x'1\cdot 1},$

$- 1 + p_{x0\cdot 0} - p_{x0\cdot 2} - 2p_{x'0\cdot 2} + 2p_{x''0\cdot 0} - p_{x''0\cdot 1} - 2p_{x''0\cdot 2} - p_{x1\cdot 1} - 2p_{x1\cdot 2} + p_{x'1\cdot 0} - p_{x'1\cdot 1},$

$- 2 + 2p_{x0\cdot 0} + p_{x1\cdot 1} + p_{x'1\cdot 0} + p_{x'1\cdot 1},$

$- 2 + p_{x0\cdot 0} + p_{x0\cdot 1} + p_{x'0\cdot 0} + 2p_{x'1\cdot 1},$

$$- 1 + p_{x0\cdot 0} + p_{x'1\cdot 1},$$
$$- 2 + p_{x0\cdot 0} + p_{x0\cdot 1} + p_{x'0\cdot 0} - p_{x'0\cdot 2} + p_{x''0\cdot 1} - p_{x''0\cdot 2} - p_{x1\cdot 2} + 2p_{x'1\cdot 1},$$
$$- 2 + 2p_{x0\cdot 0} - p_{x'0\cdot 2} + p_{x''0\cdot 0} - p_{x''0\cdot 2} + p_{x1\cdot 1} - p_{x1\cdot 2} + p_{x'1\cdot 0} + p_{x'1\cdot 1},$$
$$- 2 + 2p_{x0\cdot 0} - p_{x0\cdot 2} - p_{x'0\cdot 2} + p_{x''0\cdot 1} - p_{x''0\cdot 2} + p_{x1\cdot 1} + p_{x'1\cdot 0} + p_{x'1\cdot 1},$$
$$- 2 + p_{x0\cdot 0} + p_{x0\cdot 1} - p_{x0\cdot 2} + p_{x'0\cdot 0} - 2p_{x'0\cdot 2} + 2p_{x''0\cdot 1} - 2p_{x''0\cdot 2} - 2p_{x1\cdot 2} + 2p_{x'1\cdot 1},$$
$$- 2 + 2p_{x0\cdot 0} - p_{x0\cdot 2} - p_{x'0\cdot 2} + p_{x''0\cdot 0} + p_{x''0\cdot 1} - p_{x''0\cdot 2} + p_{x1\cdot 1} - p_{x1\cdot 2} + p_{x'1\cdot 0} + p_{x'1\cdot 1},$$
$$- 1 + p_{x0\cdot 0} - p_{x0\cdot 2} - p_{x'0\cdot 0} - p_{x'0\cdot 2} - p_{x''0\cdot 0} + p_{x''0\cdot 1} - p_{x''0\cdot 2} - p_{x1\cdot 0} + p_{x'1\cdot 1},$$
$$- 1 + p_{x0\cdot 0} - p_{x0\cdot 2} - p_{x'0\cdot 2} + p_{x''0\cdot 1} - p_{x''0\cdot 2} - p_{x1\cdot 2} + p_{x'1\cdot 1},$$
$$- 1 + p_{x0\cdot 0} - p_{x0\cdot 2} - 2p_{x'0\cdot 2} + p_{x''0\cdot 0} + p_{x''0\cdot 1} - 2p_{x''0\cdot 2} - 2p_{x1\cdot 2} + p_{x'1\cdot 1} - p_{x'1\cdot 2},$$
$$- 2 + p_{x0\cdot 0} + p_{x0\cdot 1} - p_{x0\cdot 2} + p_{x'0\cdot 0} - 2p_{x'0\cdot 2} + p_{x''0\cdot 0} + 2p_{x''0\cdot 1} - 2p_{x''0\cdot 2} - 2p_{x1\cdot 2} + 2p_{x'1\cdot 1} - p_{x'1\cdot 2},$$
$$- 2 + 2p_{x0\cdot 0} - p_{x0\cdot 2} - 2p_{x'0\cdot 2} + 2p_{x''0\cdot 0} + p_{x''0\cdot 1} - 2p_{x''0\cdot 2} + p_{x1\cdot 1} - 2p_{x1\cdot 2} + p_{x'1\cdot 0} + p_{x'1\cdot 1} - p_{x'1\cdot 2},$$
$$- 1 + p_{x0\cdot 1} - p_{x0\cdot 2} - p_{x'0\cdot 0} - p_{x'0\cdot 2} - p_{x''0\cdot 0} + 2p_{x''0\cdot 1} - p_{x''0\cdot 2} - p_{x1\cdot 0} - p_{x1\cdot 2} - p_{x'1\cdot 0} + p_{x'1\cdot 1},$$
$$- 1 + p_{x0\cdot 1} - p_{x0\cdot 2} - 2p_{x'0\cdot 0} - p_{x'0\cdot 2} - 2p_{x''0\cdot 0} + 2p_{x''0\cdot 1} - p_{x''0\cdot 2} - 2p_{x1\cdot 0} - p_{x'1\cdot 0} + p_{x'1\cdot 1},$$
$$- 1 + p_{x0\cdot 1} - p_{x0\cdot 2} - 2p_{x'0\cdot 2} - p_{x''0\cdot 0} + 2p_{x''0\cdot 1} - 2p_{x''0\cdot 2} - p_{x1\cdot 0} - 2p_{x1\cdot 2} - p_{x'1\cdot 0} + p_{x'1\cdot 1},$$
$$- 1 + p_{x0\cdot 2} - p_{x'0\cdot 1} - p_{x''0\cdot 1} + p_{x''0\cdot 2} - p_{x1\cdot 1} + p_{x'1\cdot 2},$$
$$- 1 + p_{x0\cdot 2} + p_{x'1\cdot 2},$$
$$- 1 + p_{x0\cdot 2} - p_{x'0\cdot 0} - p_{x''0\cdot 0} + p_{x''0\cdot 2} - p_{x1\cdot 0} + p_{x'1\cdot 2},$$
$$- 1 + p_{x0\cdot 0} - p_{x'0\cdot 2} + p_{x''0\cdot 0} - p_{x''0\cdot 2} - p_{x1\cdot 2} + p_{x'1\cdot 0},$$
$$- 1 + p_{x0\cdot 0} - p_{x'0\cdot 1} + p_{x''0\cdot 0} - p_{x''0\cdot 1} - p_{x1\cdot 1} + p_{x'1\cdot 0},$$
$$- 1 + p_{x0\cdot 0} + p_{x'1\cdot 0},$$
$$- 1 + p_{x0\cdot 1} - p_{x'0\cdot 0} - p_{x''0\cdot 0} + p_{x''0\cdot 1} - p_{x1\cdot 0} + p_{x'1\cdot 1},$$
$$- 1 + p_{x0\cdot 1} + p_{x'1\cdot 1},$$
$$- 1 + p_{x0\cdot 1} - p_{x'0\cdot 2} + p_{x''0\cdot 1} - p_{x''0\cdot 2} - p_{x1\cdot 2} + p_{x'1\cdot 1},$$
$$- 1 - p_{x0\cdot 1} + p_{x0\cdot 2} - 2p_{x'0\cdot 1} - p_{x''0\cdot 0} - 2p_{x''0\cdot 1} + 2p_{x''0\cdot 2} - p_{x1\cdot 0} - 2p_{x1\cdot 1} - p_{x'1\cdot 0} + p_{x'1\cdot 2},$$
$$- 1 - p_{x0\cdot 1} + p_{x0\cdot 2} - 2p_{x'0\cdot 0} - p_{x'0\cdot 1} - 2p_{x''0\cdot 0} - p_{x''0\cdot 1} + 2p_{x''0\cdot 2} - 2p_{x1\cdot 0} - p_{x'1\cdot 0} + p_{x'1\cdot 2},$$
$$- 1 - p_{x0\cdot 1} + p_{x0\cdot 2} - p_{x'0\cdot 0} - p_{x'0\cdot 1} - p_{x''0\cdot 0} - p_{x''0\cdot 1} + 2p_{x''0\cdot 2} - p_{x1\cdot 0} - p_{x1\cdot 1} - p_{x'1\cdot 0} + p_{x'1\cdot 2},$$
$$- 2 + p_{x0\cdot 0} + p_{x0\cdot 1} + p_{x1\cdot 2} + p_{x'1\cdot 1} + p_{x'1\cdot 2},$$
$$- 2 + p_{x0\cdot 0} + p_{x0\cdot 1} + p_{x'0\cdot 0} + p_{x'1\cdot 1} + p_{x'1\cdot 2},$$
$$- 3 + p_{x0\cdot 0} + 2p_{x0\cdot 1} + p_{x'0\cdot 0} + p_{x1\cdot 2} + 2p_{x'1\cdot 1} + p_{x'1\cdot 2},$$
$$- 3 + p_{x0\cdot 0} + 2p_{x0\cdot 2} + p_{x'0\cdot 0} + p_{x1\cdot 1} + p_{x'1\cdot 1} + 2p_{x'1\cdot 2},$$
$$- 2 + p_{x0\cdot 0} + p_{x0\cdot 2} + p_{x'0\cdot 0} + p_{x'1\cdot 1} + p_{x'1\cdot 2},$$
$$- 2 + p_{x0\cdot 0} + p_{x0\cdot 2} + p_{x1\cdot 1} + p_{x'1\cdot 1} + p_{x'1\cdot 2},$$
$$- 2 + p_{x0\cdot 0} + p_{x0\cdot 1} - p_{x'0\cdot 0} - p_{x''0\cdot 0} + p_{x''0\cdot 1} - p_{x1\cdot 0} + p_{x1\cdot 2} + p_{x'1\cdot 1} + p_{x'1\cdot 2},$$
$$- 2 + p_{x0\cdot 0} + p_{x0\cdot 1} + p_{x'0\cdot 0} - p_{x'0\cdot 2} + p_{x''0\cdot 1} - p_{x''0\cdot 2} - p_{x1\cdot 2} + p_{x'1\cdot 1} + p_{x'1\cdot 2},$$
$$- 2 + p_{x0\cdot 0} + p_{x0\cdot 2} + p_{x'0\cdot 0} - p_{x'0\cdot 1} - p_{x''0\cdot 1} + p_{x''0\cdot 2} - p_{x1\cdot 1} + p_{x'1\cdot 1} + p_{x'1\cdot 2},$$
$$- 2 + p_{x0\cdot 0} + p_{x0\cdot 2} - p_{x'0\cdot 0} - p_{x''0\cdot 0} + p_{x''0\cdot 2} - p_{x1\cdot 0} + p_{x1\cdot 1} + p_{x'1\cdot 1} + p_{x'1\cdot 2},$$
$$- 2 + 2p_{x0\cdot 0} - p_{x0\cdot 1} - 2p_{x'0\cdot 1} + 2p_{x''0\cdot 0} - 2p_{x''0\cdot 1} + p_{x''0\cdot 2} - 2p_{x1\cdot 1} + p_{x1\cdot 2} + p_{x'1\cdot 0} - p_{x'1\cdot 1} + p_{x'1\cdot 2},$$

$$-2+p_{x0\cdot0}-p_{x0\cdot1}+p_{x0\cdot2}+p_{x'0\cdot0}-2p_{x'0\cdot1}+p_{x''0\cdot0}-2p_{x''0\cdot1}+2p_{x''0\cdot2}-2p_{x1\cdot1}-p_{x'1\cdot1}+2p_{x'1\cdot2},$$
$$-1+p_{x0\cdot0}-p_{x0\cdot1}-p_{x'0\cdot1}-p_{x''0\cdot1}+p_{x''0\cdot2}-p_{x1\cdot1}+p_{x'1\cdot2},$$
$$-1+p_{x0\cdot0}-p_{x0\cdot1}-p_{x'0\cdot0}-p_{x'0\cdot1}-p_{x''0\cdot0}-p_{x''0\cdot1}+p_{x''0\cdot2}-p_{x1\cdot0}+p_{x'1\cdot2},$$
$$-2+2p_{x0\cdot0}-p_{x0\cdot1}-p_{x'0\cdot1}+p_{x''0\cdot0}-p_{x''0\cdot1}+p_{x''0\cdot2}-p_{x1\cdot1}+p_{x1\cdot2}+p_{x'1\cdot0}+p_{x'1\cdot2},$$
$$-2+p_{x0\cdot0}-p_{x0\cdot1}+p_{x0\cdot2}+p_{x'0\cdot0}-2p_{x'0\cdot1}-2p_{x''0\cdot1}+2p_{x''0\cdot2}-2p_{x1\cdot1}+2p_{x'1\cdot2},$$
$$-2+2p_{x0\cdot0}-p_{x0\cdot1}-p_{x'0\cdot1}-p_{x''0\cdot1}+p_{x''0\cdot2}+p_{x1\cdot2}+p_{x'1\cdot0}+p_{x'1\cdot2},$$
$$-2+p_{x0\cdot0}+p_{x0\cdot2}+p_{x'0\cdot0}-p_{x'0\cdot1}-p_{x''0\cdot1}+p_{x''0\cdot2}-p_{x1\cdot1}+2p_{x'1\cdot2},$$
$$-2+2p_{x0\cdot0}-p_{x'0\cdot1}+p_{x''0\cdot0}-p_{x''0\cdot1}-p_{x1\cdot1}+p_{x1\cdot2}+p_{x'1\cdot0}+p_{x'1\cdot2},$$
$$-2+2p_{x0\cdot0}+p_{x1\cdot2}+p_{x'1\cdot0}+p_{x'1\cdot2},$$
$$-2+p_{x0\cdot0}+p_{x0\cdot2}+p_{x'0\cdot0}+2p_{x'1\cdot2},$$
$$-1+p_{x0\cdot0}+p_{x'1\cdot2},$$
$$-1+p_{x0\cdot0}-p_{x0\cdot1}-2p_{x'0\cdot1}+p_{x''0\cdot0}-2p_{x''0\cdot1}+p_{x''0\cdot2}-2p_{x1\cdot1}-p_{x'1\cdot1}+p_{x'1\cdot2},$$
$$-1-p_{x0\cdot0}+p_{x0\cdot2}-2p_{x'0\cdot0}-2p_{x''0\cdot0}-p_{x''0\cdot1}+2p_{x''0\cdot2}-2p_{x1\cdot0}-p_{x1\cdot1}-p_{x'1\cdot1}+p_{x'1\cdot2},$$
$$-1-p_{x0\cdot0}+p_{x0\cdot2}-p_{x'0\cdot0}-2p_{x'0\cdot1}-p_{x''0\cdot0}-2p_{x''0\cdot1}+2p_{x''0\cdot2}-2p_{x1\cdot1}-p_{x'1\cdot1}+p_{x'1\cdot2},$$
$$-1-p_{x0\cdot0}+p_{x0\cdot2}-p_{x'0\cdot0}-p_{x'0\cdot1}-p_{x''0\cdot0}-p_{x''0\cdot1}+2p_{x''0\cdot2}-p_{x1\cdot0}-p_{x1\cdot1}-p_{x'1\cdot1}+p_{x'1\cdot2},$$
$$-2+p_{x0\cdot0}+p_{x0\cdot1}+p_{x1\cdot2}+p_{x'1\cdot0}+p_{x'1\cdot2},$$
$$-2+p_{x0\cdot0}+p_{x0\cdot1}+p_{x'0\cdot1}+p_{x'1\cdot0}+p_{x'1\cdot2},$$
$$-3+2p_{x0\cdot0}+p_{x0\cdot1}+p_{x'0\cdot1}+p_{x1\cdot2}+2p_{x'1\cdot0}+p_{x'1\cdot2},$$
$$-3+p_{x0\cdot1}+2p_{x0\cdot2}+p_{x'0\cdot1}+p_{x1\cdot0}+p_{x'1\cdot0}+2p_{x'1\cdot2},$$
$$-2+p_{x0\cdot1}+p_{x0\cdot2}+p_{x1\cdot0}+p_{x'1\cdot0}+p_{x'1\cdot2},$$
$$-2+p_{x0\cdot1}+p_{x0\cdot2}+p_{x'0\cdot1}+p_{x'1\cdot0}+p_{x'1\cdot2},$$
$$-2+p_{x0\cdot0}+p_{x0\cdot1}+p_{x'0\cdot1}-p_{x'0\cdot2}+p_{x''0\cdot0}-p_{x''0\cdot2}-p_{x1\cdot2}+p_{x'1\cdot0}+p_{x'1\cdot2},$$
$$-2+p_{x0\cdot0}+p_{x0\cdot1}-p_{x'0\cdot1}+p_{x''0\cdot0}-p_{x''0\cdot1}-p_{x1\cdot1}+p_{x1\cdot2}+p_{x'1\cdot0}+p_{x'1\cdot2},$$
$$-2+p_{x0\cdot1}+p_{x0\cdot2}-p_{x'0\cdot1}-p_{x''0\cdot1}+p_{x''0\cdot2}+p_{x1\cdot0}-p_{x1\cdot1}+p_{x'1\cdot0}+p_{x'1\cdot2},$$
$$-2+p_{x0\cdot1}+p_{x0\cdot2}-p_{x'0\cdot0}+p_{x'0\cdot1}-p_{x''0\cdot0}+p_{x''0\cdot2}-p_{x1\cdot0}+p_{x'1\cdot0}+p_{x'1\cdot2},$$
$$-2-p_{x0\cdot0}+2p_{x0\cdot1}-2p_{x'0\cdot0}-2p_{x''0\cdot0}+2p_{x''0\cdot1}+p_{x''0\cdot2}-2p_{x1\cdot0}+p_{x1\cdot2}-p_{x'1\cdot0}+p_{x'1\cdot1}+p_{x'1\cdot2},$$
$$-2-p_{x0\cdot0}+p_{x0\cdot1}+p_{x0\cdot2}-2p_{x'0\cdot0}+p_{x'0\cdot1}-2p_{x''0\cdot0}+p_{x''0\cdot1}+2p_{x''0\cdot2}-2p_{x1\cdot0}-p_{x'1\cdot0}+2p_{x'1\cdot2},$$
$$-1-p_{x0\cdot0}+p_{x0\cdot1}-p_{x'0\cdot0}-p_{x'0\cdot1}-p_{x''0\cdot0}-p_{x''0\cdot1}+p_{x''0\cdot2}-p_{x1\cdot1}+p_{x'1\cdot2},$$
$$-1-p_{x0\cdot0}+p_{x0\cdot1}-p_{x'0\cdot0}-p_{x''0\cdot0}+p_{x''0\cdot2}-p_{x1\cdot0}+p_{x'1\cdot2},$$
$$-2-p_{x0\cdot0}+2p_{x0\cdot1}-p_{x'0\cdot0}-p_{x''0\cdot0}+p_{x''0\cdot1}+p_{x''0\cdot2}-p_{x1\cdot0}+p_{x1\cdot2}+p_{x'1\cdot1}+p_{x'1\cdot2},$$
$$-2-p_{x0\cdot0}+p_{x0\cdot1}+p_{x0\cdot2}-2p_{x'0\cdot0}+p_{x'0\cdot1}-2p_{x''0\cdot0}+2p_{x''0\cdot2}-2p_{x1\cdot0}+2p_{x'1\cdot2},$$
$$-2-p_{x0\cdot0}+2p_{x0\cdot1}-p_{x'0\cdot0}-p_{x''0\cdot0}+p_{x''0\cdot2}+p_{x1\cdot2}+p_{x'1\cdot1}+p_{x'1\cdot2},$$
$$-2+p_{x0\cdot1}+p_{x0\cdot2}-p_{x'0\cdot0}+p_{x'0\cdot1}-p_{x''0\cdot0}+p_{x''0\cdot2}-p_{x1\cdot0}+2p_{x'1\cdot2},$$
$$-2+2p_{x0\cdot1}-p_{x'0\cdot0}-p_{x''0\cdot0}+p_{x''0\cdot1}-p_{x1\cdot0}+p_{x1\cdot2}+p_{x'1\cdot1}+p_{x'1\cdot2},$$
$$-2+2p_{x0\cdot1}+p_{x1\cdot2}+p_{x'1\cdot1}+p_{x'1\cdot2},$$
$$-2+p_{x0\cdot1}+p_{x0\cdot2}+p_{x'0\cdot1}+2p_{x'1\cdot2},$$
$$-1+p_{x0\cdot1}+p_{x'1\cdot2},$$

$$- 1 - p_{x0\cdot 0} + p_{x0\cdot 1} - 2p_{x'0\cdot 0} - 2p_{x''0\cdot 0} + p_{x''0\cdot 1} + p_{x''0\cdot 2} - 2p_{x1\cdot 0} - p_{x'1\cdot 0} + p_{x'1\cdot 2},$$
$$- 2 + 2p_{x0\cdot 1} - 2p_{x'0\cdot 0} - 2p_{x''0\cdot 0} + 2p_{x''0\cdot 1} - 2p_{x1\cdot 0} + p_{x1\cdot 2} - p_{x'1\cdot 0} + p_{x'1\cdot 1} + p_{x'1\cdot 2},$$
$$- 2 + p_{x0\cdot 1} + p_{x0\cdot 2} + p_{x'0\cdot 1} - p_{x''0\cdot 0} + p_{x''0\cdot 1} - p_{x1\cdot 0} - p_{x'1\cdot 0} + 2p_{x'1\cdot 2},$$
$$- 1 + p_{x0\cdot 1} - p_{x'0\cdot 2} - p_{x''0\cdot 0} + p_{x''0\cdot 1} - p_{x''0\cdot 2} - p_{x1\cdot 0} - p_{x1\cdot 2} - p_{x'1\cdot 0} + p_{x'1\cdot 2},$$
$$- 1 + p_{x0\cdot 1} - p_{x'0\cdot 0} - p_{x''0\cdot 0} + p_{x''0\cdot 1} - p_{x1\cdot 0} - p_{x'1\cdot 0} + p_{x'1\cdot 2},$$
$$- 2 + p_{x0\cdot 1} + p_{x0\cdot 2} - p_{x'0\cdot 0} + p_{x'0\cdot 1} - p_{x''0\cdot 0} + p_{x''0\cdot 1} + p_{x''0\cdot 2} - p_{x1\cdot 0} - p_{x'1\cdot 0} + 2p_{x'1\cdot 2},$$
$$- 1 - p_{x0\cdot 0} + p_{x0\cdot 1} - 2p_{x'0\cdot 0} - 2p_{x''0\cdot 0} + 2p_{x''0\cdot 1} - p_{x''0\cdot 2} - 2p_{x1\cdot 0} - p_{x1\cdot 2} + p_{x'1\cdot 1} - p_{x'1\cdot 2},$$
$$- 1 - p_{x0\cdot 0} + p_{x0\cdot 1} - p_{x'0\cdot 0} - 2p_{x'0\cdot 2} - p_{x''0\cdot 0} + 2p_{x''0\cdot 1} - 2p_{x''0\cdot 2} - 2p_{x1\cdot 2} + p_{x'1\cdot 1} - p_{x'1\cdot 2},$$
$$- 1 - p_{x0\cdot 0} + p_{x0\cdot 1} - p_{x'0\cdot 0} - p_{x'0\cdot 2} - p_{x''0\cdot 0} + 2p_{x''0\cdot 1} - p_{x''0\cdot 2} - p_{x1\cdot 0} - p_{x1\cdot 2} + p_{x'1\cdot 1} - p_{x'1\cdot 2},$$
$$- 2 + 2p_{x0\cdot 1} - 2p_{x'0\cdot 2} + 2p_{x''0\cdot 1} - 2p_{x''0\cdot 2} + p_{x1\cdot 0} - 2p_{x1\cdot 2} + p_{x'1\cdot 0} + p_{x'1\cdot 1} - p_{x'1\cdot 2},$$
$$- 2 + p_{x0\cdot 0} + p_{x0\cdot 1} + p_{x'0\cdot 1} + p_{x''0\cdot 1} - p_{x''0\cdot 2} - p_{x1\cdot 2} + 2p_{x'1\cdot 0} - p_{x'1\cdot 2},$$
$$- 2 + p_{x0\cdot 0} + p_{x0\cdot 1} + p_{x'0\cdot 1} - p_{x'0\cdot 2} + p_{x''0\cdot 0} + p_{x''0\cdot 1} - p_{x''0\cdot 2} - p_{x1\cdot 2} + 2p_{x'1\cdot 0} - p_{x'1\cdot 2},$$
$$- 1 + p_{x0\cdot 1} - p_{x'0\cdot 2} + p_{x''0\cdot 1} - p_{x''0\cdot 2} - p_{x1\cdot 2} + p_{x'1\cdot 0} - p_{x'1\cdot 2},$$
$$- 1 + p_{x0\cdot 1} - p_{x'0\cdot 0} - p_{x''0\cdot 0} + p_{x''0\cdot 1} - p_{x''0\cdot 2} - p_{x1\cdot 0} - p_{x1\cdot 2} + p_{x'1\cdot 0} - p_{x'1\cdot 2},$$
$$- 2 + p_{x0\cdot 0} + p_{x0\cdot 2} + p_{x1\cdot 1} + p_{x'1\cdot 0} + p_{x'1\cdot 1},$$
$$- 2 + p_{x0\cdot 0} + p_{x0\cdot 2} + p_{x'0\cdot 2} + p_{x'1\cdot 0} + p_{x'1\cdot 1},$$
$$- 3 + 2p_{x0\cdot 0} + p_{x0\cdot 2} + p_{x'0\cdot 2} + p_{x1\cdot 1} + 2p_{x'1\cdot 0} + p_{x'1\cdot 1},$$
$$- 3 + 2p_{x0\cdot 1} + p_{x0\cdot 2} + p_{x'0\cdot 2} + p_{x1\cdot 0} + p_{x'1\cdot 0} + 2p_{x'1\cdot 1},$$
$$- 2 + p_{x0\cdot 1} + p_{x0\cdot 2} + p_{x1\cdot 0} + p_{x'1\cdot 0} + p_{x'1\cdot 1},$$
$$- 2 + p_{x0\cdot 1} + p_{x0\cdot 2} + p_{x'0\cdot 2} + p_{x'1\cdot 0} + p_{x'1\cdot 1},$$
$$- 2 + p_{x0\cdot 0} + p_{x0\cdot 2} - p_{x'0\cdot 2} + p_{x''0\cdot 0} - p_{x''0\cdot 2} + p_{x1\cdot 1} - p_{x1\cdot 2} + p_{x'1\cdot 0} + p_{x'1\cdot 1},$$
$$- 2 + p_{x0\cdot 0} + p_{x0\cdot 2} - p_{x'0\cdot 1} + p_{x'0\cdot 2} + p_{x''0\cdot 0} - p_{x''0\cdot 1} - p_{x1\cdot 1} + p_{x'1\cdot 0} + p_{x'1\cdot 1},$$
$$- 2 + p_{x0\cdot 1} + p_{x0\cdot 2} - p_{x'0\cdot 2} + p_{x''0\cdot 1} - p_{x''0\cdot 2} + p_{x1\cdot 0} - p_{x1\cdot 2} + p_{x'1\cdot 0} + p_{x'1\cdot 1},$$
$$- 2 + p_{x0\cdot 1} + p_{x0\cdot 2} - p_{x'0\cdot 0} + p_{x'0\cdot 2} - p_{x''0\cdot 0} + p_{x''0\cdot 1} - p_{x1\cdot 0} + p_{x'1\cdot 0} + p_{x'1\cdot 1},$$
$$- 2 - p_{x0\cdot 0} + 2p_{x0\cdot 2} - 2p_{x'0\cdot 0} - 2p_{x''0\cdot 0} + p_{x''0\cdot 1} + 2p_{x''0\cdot 2} - 2p_{x1\cdot 0} + p_{x1\cdot 1} - p_{x'1\cdot 0} + p_{x'1\cdot 1} + p_{x'1\cdot 2},$$
$$- 2 - p_{x0\cdot 0} + p_{x0\cdot 1} + p_{x0\cdot 2} - 2p_{x'0\cdot 0} + p_{x'0\cdot 2} - 2p_{x''0\cdot 0} + 2p_{x''0\cdot 1} + p_{x''0\cdot 2} - 2p_{x1\cdot 0} - p_{x'1\cdot 0} + 2p_{x'1\cdot 1},$$
$$- 2 - p_{x0\cdot 0} + 2p_{x0\cdot 2} - p_{x'0\cdot 0} - p_{x''0\cdot 0} + p_{x''0\cdot 1} + p_{x''0\cdot 2} - p_{x1\cdot 0} + p_{x1\cdot 1} + p_{x'1\cdot 1} + p_{x'1\cdot 2},$$
$$- 1 - p_{x0\cdot 0} + p_{x0\cdot 2} - p_{x'0\cdot 0} - p_{x''0\cdot 0} + p_{x''0\cdot 1} - p_{x1\cdot 0} + p_{x'1\cdot 1},$$
$$- 1 - p_{x0\cdot 0} + p_{x0\cdot 2} - p_{x'0\cdot 0} - p_{x'0\cdot 2} - p_{x''0\cdot 0} + p_{x''0\cdot 1} - p_{x''0\cdot 2} - p_{x1\cdot 2} + p_{x'1\cdot 1},$$
$$- 2 - p_{x0\cdot 0} + p_{x0\cdot 1} + p_{x0\cdot 2} - 2p_{x'0\cdot 0} + p_{x'0\cdot 2} - 2p_{x''0\cdot 0} + 2p_{x''0\cdot 1} - 2p_{x1\cdot 0} + 2p_{x'1\cdot 1},$$
$$- 2 - p_{x0\cdot 0} + 2p_{x0\cdot 2} - p_{x'0\cdot 0} - p_{x''0\cdot 0} + p_{x''0\cdot 1} + p_{x1\cdot 1} + p_{x'1\cdot 1} + p_{x'1\cdot 2},$$
$$- 2 + p_{x0\cdot 1} + p_{x0\cdot 2} - p_{x'0\cdot 0} + p_{x'0\cdot 2} - p_{x''0\cdot 0} + p_{x''0\cdot 1} - p_{x1\cdot 0} + 2p_{x'1\cdot 1},$$
$$- 2 + 2p_{x0\cdot 2} - p_{x'0\cdot 0} - p_{x''0\cdot 0} + p_{x''0\cdot 2} - p_{x1\cdot 0} + p_{x1\cdot 1} + p_{x'1\cdot 1} + p_{x'1\cdot 2},$$
$$- 2 + 2p_{x0\cdot 2} + p_{x1\cdot 1} + p_{x'1\cdot 1} + p_{x'1\cdot 2},$$
$$- 2 + p_{x0\cdot 1} + p_{x0\cdot 2} + p_{x'0\cdot 2} + 2p_{x'1\cdot 1},$$
$$- 1 + p_{x0\cdot 2} + p_{x'1\cdot 1},$$
$$- 2 + 2p_{x0\cdot 2} - 2p_{x'0\cdot 0} - 2p_{x''0\cdot 0} + 2p_{x''0\cdot 2} - 2p_{x1\cdot 0} + p_{x1\cdot 1} - p_{x'1\cdot 0} + p_{x'1\cdot 1} + p_{x'1\cdot 2},$$

$$-2+p_{x0\cdot1}+p_{x0\cdot2}+p_{x'0\cdot2}-p_{x''0\cdot0}+p_{x''0\cdot2}-p_{x1\cdot0}-p_{x'1\cdot0}+2p_{x'1\cdot1},$$
$$-2+p_{x0\cdot1}+p_{x0\cdot2}-p_{x'0\cdot0}+p_{x'0\cdot2}-p_{x''0\cdot0}+p_{x''0\cdot1}+p_{x''0\cdot2}-p_{x1\cdot0}-p_{x'1\cdot0}+2p_{x'1\cdot1},$$
$$-1+p_{x0\cdot2}-p_{x'0\cdot1}-p_{x''0\cdot0}-p_{x''0\cdot1}+p_{x''0\cdot2}-p_{x1\cdot0}-p_{x1\cdot1}-p_{x'1\cdot0}+p_{x'1\cdot1},$$
$$-1+p_{x0\cdot2}-p_{x'0\cdot0}-p_{x''0\cdot0}+p_{x''0\cdot2}-p_{x1\cdot0}-p_{x'1\cdot0}+p_{x'1\cdot1},$$
$$-1-p_{x0\cdot0}+p_{x0\cdot2}-2p_{x'0\cdot0}-2p_{x''0\cdot0}+p_{x''0\cdot1}+p_{x''0\cdot2}-2p_{x1\cdot0}-p_{x'1\cdot0}+p_{x'1\cdot1}\}$$

$$\le \max\{2-p_{x0\cdot0}+p_{x0\cdot2}-p_{x'0\cdot0}-p_{x'0\cdot1}-p_{x''0\cdot1}+p_{x''0\cdot2}-2p_{x1\cdot1}+p_{x'1\cdot2},$$
$$2+p_{x0\cdot2}-2p_{x'0\cdot0}-p_{x''0\cdot0}+p_{x''0\cdot2}-p_{x1\cdot0}-p_{x1\cdot1}-p_{x'1\cdot1}+p_{x'1\cdot2},$$
$$2+2p_{x0\cdot2}-2p_{x'0\cdot0}-2p_{x''0\cdot0}+2p_{x''0\cdot2}-p_{x1\cdot0}-p_{x1\cdot1}+p_{x1\cdot2}-p_{x'1\cdot1}+2p_{x'1\cdot2},$$
$$2-p_{x0\cdot0}-p_{x'0\cdot0}-p_{x'0\cdot1}-p_{x''0\cdot0}+p_{x''0\cdot2}-2p_{x1\cdot1}+p_{x1\cdot2}+p_{x'1\cdot2},$$
$$2-p_{x0\cdot0}+p_{x0\cdot2}-p_{x'0\cdot0}-p_{x'0\cdot1}-p_{x''0\cdot0}-p_{x''0\cdot1}+p_{x''0\cdot2}-2p_{x1\cdot1}+p_{x1\cdot2}+p_{x'1\cdot2},$$
$$1+p_{x0\cdot2}-p_{x'0\cdot0}-p_{x''0\cdot0}+p_{x''0\cdot2}-p_{x1\cdot1}+p_{x1\cdot2}+p_{x'1\cdot2},$$
$$1+p_{x0\cdot1}-p_{x'0\cdot0}-p_{x''0\cdot0}+p_{x''0\cdot1}+p_{x''0\cdot2}-p_{x1\cdot1}+p_{x1\cdot2}+p_{x'1\cdot1}+p_{x'1\cdot2},$$
$$2+p_{x0\cdot2}-p_{x'0\cdot0}-p_{x'0\cdot2}-p_{x''0\cdot0}+p_{x''0\cdot2}-p_{x1\cdot0}-p_{x1\cdot1}-p_{x'1\cdot1}+p_{x'1\cdot2},$$
$$2+p_{x0\cdot1}-p_{x0\cdot2}-p_{x'0\cdot0}-p_{x'0\cdot2}-p_{x''0\cdot0}+p_{x''0\cdot1}-p_{x1\cdot0}-p_{x1\cdot1}+p_{x'1\cdot1},$$
$$1-p_{x'0\cdot2}-p_{x1\cdot1},$$
$$2-2p_{x'0\cdot2}-p_{x1\cdot1}-p_{x1\cdot2}-p_{x'1\cdot1},$$
$$2-p_{x0\cdot2}-p_{x'0\cdot1}-p_{x'0\cdot2}-2p_{x1\cdot1},$$
$$2+p_{x0\cdot0}-p_{x0\cdot2}-p_{x'0\cdot1}-p_{x'0\cdot2}+p_{x''0\cdot0}-p_{x''0\cdot1}-2p_{x1\cdot1}+p_{x'1\cdot0},$$
$$2+p_{x0\cdot0}-2p_{x'0\cdot2}+p_{x''0\cdot0}-p_{x''0\cdot2}-p_{x1\cdot1}-p_{x1\cdot2}+p_{x'1\cdot0}-p_{x'1\cdot1},$$
$$1+p_{x0\cdot1}-p_{x'0\cdot2}+p_{x''0\cdot0}+p_{x''0\cdot1}-p_{x''0\cdot2}+p_{x1\cdot0}-p_{x1\cdot1}+p_{x'1\cdot0}+p_{x'1\cdot1},$$
$$1+p_{x0\cdot0}-p_{x'0\cdot2}+p_{x''0\cdot0}-p_{x''0\cdot2}+p_{x1\cdot0}-p_{x1\cdot1}+p_{x'1\cdot0},$$
$$2+p_{x0\cdot0}-p_{x0\cdot2}-p_{x'0\cdot1}-p_{x'0\cdot2}+p_{x''0\cdot0}-p_{x''0\cdot1}-p_{x''0\cdot2}+p_{x1\cdot0}-2p_{x1\cdot1}+p_{x'1\cdot0},$$
$$2-p_{x0\cdot2}-p_{x'0\cdot1}-p_{x'0\cdot2}+p_{x''0\cdot0}-p_{x''0\cdot2}+p_{x1\cdot0}-2p_{x1\cdot1}+p_{x'1\cdot0},$$
$$2+2p_{x0\cdot0}-2p_{x'0\cdot2}+2p_{x''0\cdot0}-2p_{x''0\cdot2}+p_{x1\cdot0}-p_{x1\cdot1}-p_{x1\cdot2}+2p_{x'1\cdot0}-p_{x'1\cdot1},$$
$$2-p_{x0\cdot0}+p_{x0\cdot1}-p_{x'0\cdot0}-p_{x'0\cdot2}+p_{x''0\cdot1}-p_{x''0\cdot2}-p_{x1\cdot1}-p_{x1\cdot2}+p_{x'1\cdot1},$$
$$2+p_{x0\cdot0}-p_{x'0\cdot0}-p_{x'0\cdot2}+p_{x''0\cdot0}-p_{x''0\cdot2}-p_{x1\cdot1}-p_{x1\cdot2}+p_{x'1\cdot0}-p_{x'1\cdot1},$$
$$2-2p_{x'0\cdot0}-p_{x1\cdot0}-p_{x1\cdot1}-p_{x'1\cdot1},$$
$$2-p_{x0\cdot0}-p_{x'0\cdot0}-p_{x'0\cdot1}-2p_{x1\cdot1},$$
$$1-p_{x'0\cdot0}-p_{x1\cdot1},$$
$$2-p_{x0\cdot0}-p_{x'0\cdot0}-p_{x'0\cdot2}-p_{x1\cdot1}-p_{x1\cdot2},$$
$$2-p_{x'0\cdot0}-p_{x'0\cdot2}-p_{x1\cdot1}-p_{x1\cdot2}-p_{x'1\cdot1},$$
$$3-p_{x0\cdot0}-p_{x'0\cdot0}-2p_{x'0\cdot2}-p_{x1\cdot1}-2p_{x1\cdot2}-p_{x'1\cdot1},$$
$$3-p_{x0\cdot2}-2p_{x'0\cdot0}-p_{x'0\cdot2}-2p_{x1\cdot0}-p_{x1\cdot1}-p_{x'1\cdot1},$$
$$2-p_{x'0\cdot0}-p_{x'0\cdot2}-p_{x1\cdot0}-p_{x1\cdot1}-p_{x'1\cdot1},$$
$$2-p_{x0\cdot2}-p_{x'0\cdot0}-p_{x'0\cdot2}-p_{x1\cdot0}-p_{x1\cdot1},$$
$$1+p_{x0\cdot0}+p_{x0\cdot2}-p_{x'0\cdot1}+p_{x'0\cdot2}+p_{x''0\cdot0}-2p_{x''0\cdot1}+p_{x''0\cdot2}+p_{x1\cdot0}-p_{x1\cdot1}+p_{x'1\cdot0}+p_{x'1\cdot2},$$

$2 + p_{x0\cdot2} - 2p_{x'0\cdot0} + p_{x'0\cdot2} - p_{x''0\cdot1} + p_{x''0\cdot2} - p_{x1\cdot0} - p_{x1\cdot1} - p_{x'1\cdot1},$

$2 - p_{x0\cdot0} + 2p_{x0\cdot2} - p_{x'0\cdot0} - p_{x'0\cdot1} + p_{x'0\cdot2} - 2p_{x''0\cdot1} + 2p_{x''0\cdot2} - 2p_{x1\cdot1} + 2p_{x'1\cdot2},$

$2 + p_{x0\cdot2} - 2p_{x'0\cdot0} + p_{x'0\cdot2} - p_{x''0\cdot0} - p_{x''0\cdot1} + p_{x''0\cdot2} - p_{x1\cdot0} - p_{x1\cdot1} - p_{x'1\cdot1} + p_{x'1\cdot2},$

$1 + p_{x0\cdot0} + p_{x0\cdot2} - p_{x'0\cdot0} + p_{x'0\cdot2} + p_{x''0\cdot0} - p_{x''0\cdot1} + p_{x''0\cdot2} - p_{x1\cdot1} + p_{x'1\cdot0},$

$1 + p_{x0\cdot2} - p_{x'0\cdot0} + p_{x'0\cdot2} - p_{x''0\cdot1} + p_{x''0\cdot2} - p_{x1\cdot1} + p_{x'1\cdot2},$

$1 + 2p_{x0\cdot2} - p_{x'0\cdot1} + p_{x'0\cdot2} + p_{x''0\cdot0} - 2p_{x''0\cdot1} + 2p_{x''0\cdot2} + p_{x1\cdot0} - p_{x1\cdot1} + p_{x'1\cdot0} + 2p_{x'1\cdot2},$

$1 + 2p_{x0\cdot0} + p_{x0\cdot2} - p_{x'0\cdot1} + p_{x'0\cdot2} + 2p_{x''0\cdot0} - 2p_{x''0\cdot1} + p_{x''0\cdot2} + p_{x1\cdot0} - p_{x1\cdot1} + 2p_{x'1\cdot0},$

$1 + 2p_{x0\cdot2} - p_{x'0\cdot0} + p_{x'0\cdot2} - p_{x''0\cdot0} - p_{x''0\cdot1} + 2p_{x''0\cdot2} - p_{x1\cdot1} + p_{x1\cdot2} + 2p_{x'1\cdot2},$

$2 - p_{x0\cdot0} + 2p_{x0\cdot2} - p_{x'0\cdot0} - p_{x'0\cdot1} + p_{x'0\cdot2} - p_{x''0\cdot0} - 2p_{x''0\cdot1} + 2p_{x''0\cdot2} - 2p_{x1\cdot1} + p_{x1\cdot2} + 2p_{x'1\cdot2},$

$2 + 2p_{x0\cdot2} - 2p_{x'0\cdot0} + p_{x'0\cdot2} - 2p_{x''0\cdot0} - p_{x''0\cdot1} + 2p_{x''0\cdot2} - p_{x1\cdot0} - p_{x1\cdot1} + p_{x1\cdot2} - p_{x'1\cdot1} + 2p_{x'1\cdot2},$

$2 + p_{x0\cdot2} - 2p_{x'0\cdot1} - p_{x''0\cdot1} + p_{x''0\cdot2} - p_{x1\cdot0} - p_{x1\cdot1} - p_{x'1\cdot0} + p_{x'1\cdot2},$

$2 - p_{x0\cdot1} + p_{x0\cdot2} - p_{x'0\cdot0} - p_{x'0\cdot1} - p_{x''0\cdot0} + p_{x''0\cdot2} - 2p_{x1\cdot0} + p_{x'1\cdot2},$

$1 + p_{x0\cdot2} - p_{x'0\cdot1} - p_{x''0\cdot1} + p_{x''0\cdot2} - p_{x1\cdot0} + p_{x1\cdot2} + p_{x'1\cdot2},$

$2 - p_{x0\cdot1} + p_{x0\cdot2} - p_{x'0\cdot0} - p_{x'0\cdot1} - p_{x''0\cdot0} - p_{x''0\cdot1} + p_{x''0\cdot2} - 2p_{x1\cdot0} + p_{x1\cdot2} + p_{x'1\cdot2},$

$1 + p_{x0\cdot0} - p_{x'0\cdot1} + p_{x''0\cdot0} - p_{x''0\cdot1} + p_{x''0\cdot2} - p_{x1\cdot0} + p_{x1\cdot2} + p_{x'1\cdot0} + p_{x'1\cdot2},$

$2 + 2p_{x0\cdot2} - 2p_{x'0\cdot1} - 2p_{x''0\cdot1} + 2p_{x''0\cdot2} - p_{x1\cdot0} - p_{x1\cdot1} + p_{x1\cdot2} - p_{x'1\cdot0} + 2p_{x'1\cdot2},$

$2 - p_{x0\cdot1} - p_{x'0\cdot0} - p_{x'0\cdot1} - p_{x''0\cdot1} + p_{x''0\cdot2} - 2p_{x1\cdot0} + p_{x1\cdot2} + p_{x'1\cdot2},$

$2 + p_{x0\cdot1} - 2p_{x'0\cdot2} + p_{x''0\cdot1} - p_{x''0\cdot2} - p_{x1\cdot0} - p_{x1\cdot2} - p_{x'1\cdot0} + p_{x'1\cdot1},$

$2 + p_{x0\cdot1} - p_{x0\cdot2} - p_{x'0\cdot0} - p_{x'0\cdot2} - p_{x''0\cdot0} + p_{x''0\cdot1} - 2p_{x1\cdot0} + p_{x'1\cdot1},$

$2 + p_{x0\cdot2} - p_{x'0\cdot1} - p_{x'0\cdot2} - p_{x''0\cdot1} + p_{x''0\cdot2} - p_{x1\cdot0} - p_{x1\cdot1} - p_{x'1\cdot0} + p_{x'1\cdot2},$

$2 + p_{x0\cdot0} - p_{x0\cdot2} - p_{x'0\cdot1} - p_{x'0\cdot2} + p_{x''0\cdot0} - p_{x''0\cdot1} - p_{x1\cdot0} - p_{x1\cdot1} + p_{x'1\cdot0},$

$2 - p_{x0\cdot2} - p_{x'0\cdot0} - p_{x'0\cdot2} - 2p_{x1\cdot0},$

$2 - 2p_{x'0\cdot2} - p_{x1\cdot0} - p_{x1\cdot2} - p_{x'1\cdot0},$

$1 - p_{x'0\cdot2} - p_{x1\cdot0},$

$2 - p_{x0\cdot2} - p_{x'0\cdot0} - p_{x'0\cdot2} + p_{x''0\cdot1} - p_{x''0\cdot2} - 2p_{x1\cdot0} + p_{x1\cdot1} + p_{x'1\cdot1},$

$2 + 2p_{x0\cdot1} - 2p_{x'0\cdot2} + 2p_{x''0\cdot1} - 2p_{x''0\cdot2} - p_{x1\cdot0} + p_{x1\cdot1} - p_{x1\cdot2} - p_{x'1\cdot0} + 2p_{x'1\cdot1},$

$1 + p_{x0\cdot1} - p_{x'0\cdot2} + p_{x''0\cdot1} - p_{x''0\cdot2} - p_{x1\cdot0} + p_{x1\cdot1} + p_{x'1\cdot1},$

$1 + p_{x0\cdot0} - p_{x'0\cdot2} + p_{x''0\cdot0} + p_{x''0\cdot1} - p_{x''0\cdot2} - p_{x1\cdot0} + p_{x1\cdot1} + p_{x'1\cdot0} + p_{x'1\cdot1},$

$2 + p_{x0\cdot1} - p_{x0\cdot2} - p_{x'0\cdot0} - p_{x'0\cdot2} - p_{x''0\cdot0} + p_{x''0\cdot1} - p_{x''0\cdot2} - 2p_{x1\cdot0} + p_{x1\cdot1} + p_{x'1\cdot1},$

$2 + p_{x0\cdot1} - p_{x'0\cdot1} - p_{x'0\cdot2} + p_{x''0\cdot1} - p_{x''0\cdot2} - p_{x1\cdot0} - p_{x1\cdot2} - p_{x'1\cdot0} + p_{x'1\cdot1},$

$2 + p_{x0\cdot0} - p_{x0\cdot1} - p_{x'0\cdot1} - p_{x'0\cdot2} + p_{x''0\cdot0} - p_{x''0\cdot2} - p_{x1\cdot0} - p_{x1\cdot2} + p_{x'1\cdot0},$

$2 - p_{x0\cdot1} - p_{x'0\cdot0} - p_{x'0\cdot1} - 2p_{x1\cdot0},$

$2 - 2p_{x'0\cdot1} - p_{x1\cdot0} - p_{x1\cdot1} - p_{x'1\cdot0},$

$1 - p_{x'0\cdot1} - p_{x1\cdot0},$

$2 - p_{x0\cdot1} - p_{x'0\cdot1} - p_{x'0\cdot2} - p_{x1\cdot0} - p_{x1\cdot2},$

$2 - p_{x'0\cdot1} - p_{x'0\cdot2} - p_{x1\cdot0} - p_{x1\cdot2} - p_{x'1\cdot0},$

$3 - p_{x0\cdot1} - p_{x'0\cdot1} - 2p_{x'0\cdot2} - p_{x1\cdot0} - 2p_{x1\cdot2} - p_{x'1\cdot0},$

$2 - p_{x'0\cdot1} - p_{x'0\cdot2} - p_{x1\cdot0} - p_{x1\cdot1} - p_{x'1\cdot0},$

$3 - p_{x0\cdot2} - 2p_{x'0\cdot1} - p_{x'0\cdot2} - p_{x1\cdot0} - 2p_{x1\cdot1} - p_{x'1\cdot0},$

$2 - p_{x0\cdot2} - p_{x'0\cdot1} - p_{x'0\cdot2} - p_{x1\cdot0} - p_{x1\cdot1},$

$1 + p_{x0\cdot1} + p_{x0\cdot2} - p_{x'0\cdot0} + p_{x'0\cdot2} - 2p_{x''0\cdot0} + p_{x''0\cdot1} + p_{x''0\cdot2} - p_{x1\cdot0} + p_{x1\cdot1} + p_{x'1\cdot1} + p_{x'1\cdot2},$

$2 - p_{x0\cdot1} + 2p_{x0\cdot2} - p_{x'0\cdot0} - p_{x'0\cdot1} + p_{x'0\cdot2} - 2p_{x''0\cdot0} + 2p_{x''0\cdot2} - 2p_{x1\cdot0} + 2p_{x'1\cdot2},$

$2 + p_{x0\cdot2} - 2p_{x'0\cdot1} + p_{x'0\cdot2} - p_{x''0\cdot0} + p_{x''0\cdot2} - p_{x1\cdot0} - p_{x1\cdot1} - p_{x'1\cdot0},$

$2 + p_{x0\cdot2} - 2p_{x'0\cdot1} + p_{x'0\cdot2} - p_{x''0\cdot0} - p_{x''0\cdot1} + p_{x''0\cdot2} - p_{x1\cdot0} - p_{x1\cdot1} - p_{x'1\cdot0} + p_{x'1\cdot2},$

$1 + p_{x0\cdot1} + p_{x0\cdot2} - p_{x'0\cdot1} + p_{x'0\cdot2} - p_{x''0\cdot0} + p_{x''0\cdot1} + p_{x''0\cdot2} - p_{x1\cdot0} + p_{x'1\cdot1},$

$1 + p_{x0\cdot2} - p_{x'0\cdot1} + p_{x'0\cdot2} - p_{x''0\cdot0} + p_{x''0\cdot2} - p_{x1\cdot0} + p_{x'1\cdot2},$

$1 + 2p_{x0\cdot2} - p_{x'0\cdot0} + p_{x'0\cdot2} - 2p_{x''0\cdot0} + p_{x''0\cdot1} + 2p_{x''0\cdot2} - p_{x1\cdot0} + p_{x1\cdot1} + p_{x'1\cdot1} + 2p_{x'1\cdot2},$

$1 + 2p_{x0\cdot1} + p_{x0\cdot2} - p_{x'0\cdot0} + p_{x'0\cdot2} - 2p_{x''0\cdot0} + 2p_{x''0\cdot1} + p_{x''0\cdot2} - p_{x1\cdot0} + p_{x1\cdot1} + 2p_{x'1\cdot1},$

$1 + 2p_{x0\cdot2} - p_{x'0\cdot1} + p_{x'0\cdot2} - p_{x''0\cdot0} - p_{x''0\cdot1} + 2p_{x''0\cdot2} - p_{x1\cdot0} + p_{x1\cdot2} + 2p_{x'1\cdot2},$

$2 + 2p_{x0\cdot2} - 2p_{x'0\cdot1} + p_{x'0\cdot2} - p_{x''0\cdot0} - 2p_{x''0\cdot1} + 2p_{x''0\cdot2} - p_{x1\cdot0} - p_{x1\cdot1} + p_{x1\cdot2} - p_{x'1\cdot0} + 2p_{x'1\cdot2},$

$2 - p_{x0\cdot1} + 2p_{x0\cdot2} - p_{x'0\cdot0} - p_{x'0\cdot1} + p_{x'0\cdot2} - 2p_{x''0\cdot0} - p_{x''0\cdot1} + 2p_{x''0\cdot2} - 2p_{x1\cdot0} + p_{x1\cdot2} + 2p_{x'1\cdot2},$

$1 + p_{x0\cdot1} + p_{x0\cdot2} - p_{x'0\cdot0} + p_{x'0\cdot1} - 2p_{x''0\cdot0} + p_{x''0\cdot1} + p_{x''0\cdot2} - p_{x1\cdot0} + p_{x1\cdot2} + p_{x'1\cdot1} + p_{x'1\cdot2},$

$2 + 2p_{x0\cdot1} - p_{x0\cdot2} - p_{x'0\cdot0} + p_{x'0\cdot1} - p_{x'0\cdot2} - 2p_{x''0\cdot0} + 2p_{x''0\cdot1} - 2p_{x1\cdot0} + 2p_{x'1\cdot1},$

$2 + p_{x0\cdot1} + p_{x'0\cdot1} - 2p_{x'0\cdot2} - p_{x''0\cdot0} + p_{x''0\cdot1} - p_{x1\cdot0} - p_{x1\cdot2} - p_{x'1\cdot0},$

$2 + p_{x0\cdot1} + p_{x'0\cdot1} - 2p_{x'0\cdot2} - p_{x''0\cdot0} + p_{x''0\cdot1} - p_{x''0\cdot2} - p_{x1\cdot0} - p_{x1\cdot2} - p_{x'1\cdot0} + p_{x'1\cdot1},$

$1 + p_{x0\cdot1} + p_{x0\cdot2} + p_{x'0\cdot1} - p_{x'0\cdot2} - p_{x''0\cdot0} + p_{x''0\cdot1} + p_{x''0\cdot2} - p_{x1\cdot0} + p_{x'1\cdot2},$

$1 + p_{x0\cdot1} + p_{x'0\cdot1} - p_{x'0\cdot2} - p_{x''0\cdot0} + p_{x''0\cdot1} - p_{x1\cdot0} + p_{x'1\cdot1},$

$1 + p_{x0\cdot1} + 2p_{x0\cdot2} - p_{x'0\cdot0} + p_{x'0\cdot1} - 2p_{x''0\cdot0} + p_{x''0\cdot1} + 2p_{x''0\cdot2} - p_{x1\cdot0} + p_{x1\cdot2} + 2p_{x'1\cdot2},$

$1 + 2p_{x0\cdot1} - p_{x'0\cdot0} + p_{x'0\cdot1} - 2p_{x''0\cdot0} + 2p_{x''0\cdot1} + p_{x''0\cdot2} - p_{x1\cdot0} + p_{x1\cdot2} + 2p_{x'1\cdot1} + p_{x'1\cdot2},$

$1 + 2p_{x0\cdot1} + p_{x'0\cdot1} - p_{x'0\cdot2} - p_{x''0\cdot0} + 2p_{x''0\cdot1} - p_{x''0\cdot2} - p_{x1\cdot0} + p_{x1\cdot1} + 2p_{x'1\cdot1},$

$2 + 2p_{x0\cdot1} + p_{x'0\cdot1} - 2p_{x'0\cdot2} - p_{x''0\cdot0} + 2p_{x''0\cdot1} - 2p_{x''0\cdot2} - p_{x1\cdot0} + p_{x1\cdot1} - p_{x1\cdot2} - p_{x'1\cdot0} + 2p_{x'1\cdot1},$

$2 + 2p_{x0\cdot1} - p_{x0\cdot2} - p_{x'0\cdot0} + p_{x'0\cdot1} - p_{x'0\cdot2} - 2p_{x''0\cdot0} + 2p_{x''0\cdot1} - p_{x''0\cdot2} - 2p_{x1\cdot0} + p_{x1\cdot1} + 2p_{x'1\cdot1},$

$1 - p_{x'0\cdot2} - p_{x1\cdot2},$

$1 - p_{x'0\cdot1} - p_{x1\cdot1},$

$1 + p_{x0\cdot1} - p_{x'0\cdot2} + p_{x''0\cdot1} - p_{x''0\cdot2} - p_{x1\cdot2} + p_{x'1\cdot1},$

$1 + p_{x0\cdot2} - p_{x'0\cdot1} - p_{x''0\cdot1} + p_{x''0\cdot2} - p_{x1\cdot1} + p_{x'1\cdot2},$

$1 - p_{x'0\cdot0} - p_{x1\cdot0},$

$1 + p_{x0\cdot0} - p_{x'0\cdot2} + p_{x''0\cdot0} - p_{x''0\cdot2} - p_{x1\cdot2} + p_{x'1\cdot0},$

$1 + p_{x0\cdot2} - p_{x'0\cdot0} - p_{x''0\cdot0} + p_{x''0\cdot2} - p_{x1\cdot0} + p_{x'1\cdot2},$

$1 + p_{x0\cdot0} - p_{x'0\cdot1} + p_{x''0\cdot0} - p_{x''0\cdot1} - p_{x1\cdot1} + p_{x'1\cdot0},$

$1 + p_{x0\cdot1} - p_{x'0\cdot0} - p_{x''0\cdot0} + p_{x''0\cdot1} - p_{x1\cdot0} + p_{x'1\cdot1},$

$2 + 2p_{x0\cdot0} - p_{x0\cdot2} + p_{x'0\cdot0} - p_{x'0\cdot1} - p_{x'0\cdot2} + 2p_{x''0\cdot0} - 2p_{x''0\cdot1} - p_{x''0\cdot2} + p_{x1\cdot0} - 2p_{x1\cdot1} + 2p_{x'1\cdot0},$

$2 + 2p_{x0\cdot0} + p_{x'0\cdot0} - 2p_{x'0\cdot2} + 2p_{x''0\cdot0} - p_{x''0\cdot1} - 2p_{x''0\cdot2} + p_{x1\cdot0} - p_{x1\cdot1} - p_{x1\cdot2} + 2p_{x'1\cdot0} - p_{x'1\cdot1},$

$1 + 2p_{x0\cdot0} + p_{x'0\cdot0} - p_{x'0\cdot2} + 2p_{x''0\cdot0} - p_{x''0\cdot1} - p_{x''0\cdot2} + p_{x1\cdot0} - p_{x1\cdot1} + 2p_{x'1\cdot0},$

$$1 + 2p_{x0\cdot0} + p_{x'0\cdot0} - p_{x'0\cdot1} + 2p_{x''0\cdot0} - 2p_{x''0\cdot1} + p_{x''0\cdot2} - p_{x1\cdot1} + p_{x1\cdot2} + 2p_{x'1\cdot0} + p_{x'1\cdot2},$$
$$1 + p_{x0\cdot0} + 2p_{x0\cdot2} + p_{x'0\cdot0} - p_{x'0\cdot1} + p_{x''0\cdot0} - 2p_{x''0\cdot1} + 2p_{x''0\cdot2} - p_{x1\cdot1} + p_{x1\cdot2} + 2p_{x'1\cdot2},$$
$$1 + p_{x0\cdot0} + p_{x0\cdot2} + p_{x'0\cdot0} - p_{x'0\cdot1} + p_{x''0\cdot0} - 2p_{x''0\cdot1} + p_{x''0\cdot2} - p_{x1\cdot1} + p_{x1\cdot2} + p_{x'1\cdot0} + p_{x'1\cdot2},$$
$$1 + p_{x0\cdot0} + p_{x'0\cdot0} - p_{x'0\cdot2} + p_{x''0\cdot0} - p_{x''0\cdot1} - p_{x1\cdot1} + p_{x'1\cdot0},$$
$$2 + p_{x0\cdot0} + p_{x'0\cdot0} - 2p_{x'0\cdot2} + p_{x''0\cdot0} - p_{x''0\cdot1} - p_{x''0\cdot2} - p_{x1\cdot1} - p_{x1\cdot2} + p_{x'1\cdot0} - p_{x'1\cdot1},$$
$$1 + p_{x0\cdot0} + p_{x0\cdot2} + p_{x'0\cdot0} - p_{x'0\cdot2} + p_{x''0\cdot0} - p_{x''0\cdot1} + p_{x''0\cdot2} - p_{x1\cdot1} + p_{x'1\cdot2},$$
$$2 + p_{x0\cdot0} + p_{x'0\cdot0} - 2p_{x'0\cdot2} + p_{x''0\cdot0} - p_{x''0\cdot1} - p_{x1\cdot1} - p_{x1\cdot2} - p_{x'1\cdot1},$$
$$2 + 2p_{x0\cdot0} - p_{x0\cdot2} + p_{x'0\cdot0} - p_{x'0\cdot1} - p_{x'0\cdot2} + 2p_{x''0\cdot0} - 2p_{x''0\cdot1} - 2p_{x1\cdot1} + 2p_{x'1\cdot0},$$
$$2 + 2p_{x0\cdot0} + p_{x'0\cdot0} - 2p_{x'0\cdot1} + 2p_{x''0\cdot0} - 2p_{x''0\cdot1} - p_{x''0\cdot2} + p_{x1\cdot0} - p_{x1\cdot1} - p_{x1\cdot2} + 2p_{x'1\cdot0} - p_{x'1\cdot2},$$
$$2 + 2p_{x0\cdot0} - p_{x0\cdot1} + p_{x'0\cdot0} - p_{x'0\cdot1} - p_{x'0\cdot2} + 2p_{x''0\cdot0} - p_{x''0\cdot1} - 2p_{x''0\cdot2} + p_{x1\cdot0} - 2p_{x1\cdot2} + 2p_{x'1\cdot0},$$
$$1 + 2p_{x0\cdot0} + p_{x'0\cdot0} - p_{x'0\cdot1} + 2p_{x''0\cdot0} - p_{x''0\cdot1} - p_{x''0\cdot2} + p_{x1\cdot0} - p_{x1\cdot2} + 2p_{x'1\cdot0},$$
$$1 + 2p_{x0\cdot0} + p_{x'0\cdot0} - p_{x'0\cdot2} + 2p_{x''0\cdot0} + p_{x''0\cdot1} - 2p_{x''0\cdot2} + p_{x1\cdot1} - p_{x1\cdot2} + 2p_{x'1\cdot0} + p_{x'1\cdot1},$$
$$1 + p_{x0\cdot0} + 2p_{x0\cdot1} + p_{x'0\cdot0} - p_{x'0\cdot2} + p_{x''0\cdot0} + 2p_{x''0\cdot1} - 2p_{x''0\cdot2} + p_{x1\cdot1} - p_{x1\cdot2} + 2p_{x'1\cdot1},$$
$$1 + p_{x0\cdot0} + p_{x0\cdot1} + p_{x'0\cdot0} - p_{x'0\cdot2} + p_{x''0\cdot0} + p_{x''0\cdot1} - 2p_{x''0\cdot2} + p_{x1\cdot1} - p_{x1\cdot2} + p_{x'1\cdot0} + p_{x'1\cdot1},$$
$$1 + p_{x0\cdot0} + p_{x'0\cdot0} - p_{x'0\cdot1} + p_{x''0\cdot0} - p_{x''0\cdot2} - p_{x1\cdot2} + p_{x'1\cdot0},$$
$$2 + p_{x0\cdot0} + p_{x'0\cdot0} - 2p_{x'0\cdot1} + p_{x''0\cdot0} - p_{x''0\cdot1} - p_{x''0\cdot2} - p_{x1\cdot1} - p_{x1\cdot2} + p_{x'1\cdot0} - p_{x'1\cdot2},$$
$$1 + p_{x0\cdot0} + p_{x0\cdot1} + p_{x'0\cdot0} - p_{x'0\cdot1} + p_{x''0\cdot0} + p_{x''0\cdot1} - p_{x''0\cdot2} - p_{x1\cdot2} + p_{x'1\cdot1},$$
$$2 + p_{x0\cdot0} + p_{x'0\cdot0} - 2p_{x'0\cdot1} + p_{x''0\cdot0} - p_{x''0\cdot2} - p_{x1\cdot1} - p_{x1\cdot2} - p_{x'1\cdot2},$$
$$2 + 2p_{x0\cdot0} - p_{x0\cdot1} + p_{x'0\cdot0} - p_{x'0\cdot1} - p_{x'0\cdot2} + 2p_{x''0\cdot0} - 2p_{x''0\cdot2} - 2p_{x1\cdot2} + 2p_{x'1\cdot0},$$
$$2 + 2p_{x0\cdot1} - 2p_{x'0\cdot0} + p_{x'0\cdot1} - 2p_{x''0\cdot0} + 2p_{x''0\cdot1} - p_{x''0\cdot2} - p_{x1\cdot0} + p_{x1\cdot1} - p_{x1\cdot2} + 2p_{x'1\cdot1} - p_{x'1\cdot2},$$
$$2 - p_{x0\cdot0} + 2p_{x0\cdot1} - p_{x'0\cdot0} + p_{x'0\cdot1} - p_{x'0\cdot2} - p_{x''0\cdot0} + 2p_{x''0\cdot1} - 2p_{x''0\cdot2} + p_{x1\cdot1} - 2p_{x1\cdot2} + 2p_{x'1\cdot1},$$
$$1 + 2p_{x0\cdot1} - p_{x'0\cdot0} + p_{x'0\cdot1} - p_{x''0\cdot0} + 2p_{x''0\cdot1} - p_{x''0\cdot2} + p_{x1\cdot1} - p_{x1\cdot2} + 2p_{x'1\cdot1},$$
$$1 + 2p_{x0\cdot0} + p_{x0\cdot1} + p_{x'0\cdot1} - p_{x'0\cdot2} + 2p_{x''0\cdot0} + p_{x''0\cdot1} - 2p_{x''0\cdot2} + p_{x1\cdot0} - p_{x1\cdot2} + 2p_{x'1\cdot0},$$
$$1 + 2p_{x0\cdot1} + p_{x'0\cdot1} - p_{x'0\cdot2} + p_{x''0\cdot0} + 2p_{x''0\cdot1} - 2p_{x''0\cdot2} + p_{x1\cdot0} - p_{x1\cdot2} + p_{x'1\cdot0} + 2p_{x'1\cdot1},$$
$$1 + p_{x0\cdot0} + p_{x0\cdot1} + p_{x'0\cdot1} - p_{x'0\cdot2} + p_{x''0\cdot0} + p_{x''0\cdot1} - 2p_{x''0\cdot2} + p_{x1\cdot0} - p_{x1\cdot2} + p_{x'1\cdot0} + p_{x'1\cdot1},$$
$$1 + p_{x0\cdot1} - p_{x'0\cdot0} + p_{x'0\cdot1} + p_{x''0\cdot1} - p_{x''0\cdot2} - p_{x1\cdot2} + p_{x'1\cdot1},$$
$$2 + p_{x0\cdot1} - 2p_{x'0\cdot0} + p_{x'0\cdot1} - p_{x''0\cdot0} + p_{x''0\cdot1} - p_{x''0\cdot2} - p_{x1\cdot0} - p_{x1\cdot2} + p_{x'1\cdot1} - p_{x'1\cdot2},$$
$$1 + p_{x0\cdot0} + p_{x0\cdot1} - p_{x'0\cdot0} + p_{x'0\cdot1} + p_{x''0\cdot0} + p_{x''0\cdot1} - p_{x''0\cdot2} - p_{x1\cdot2} + p_{x'1\cdot0},$$
$$2 - p_{x0\cdot0} + 2p_{x0\cdot1} - p_{x'0\cdot0} + p_{x'0\cdot1} - p_{x'0\cdot2} + 2p_{x''0\cdot1} - 2p_{x''0\cdot2} - 2p_{x1\cdot2} + 2p_{x'1\cdot1},$$
$$2 + p_{x0\cdot1} - 2p_{x'0\cdot0} + p_{x'0\cdot1} + p_{x''0\cdot1} - p_{x''0\cdot2} - p_{x1\cdot0} - p_{x1\cdot2} - p_{x'1\cdot2},$$
$$2 - p_{x0\cdot1} - p_{x'0\cdot0} - p_{x'0\cdot1} - p_{x1\cdot0} - p_{x1\cdot2},$$
$$2 - p_{x'0\cdot0} - p_{x'0\cdot1} - p_{x1\cdot0} - p_{x1\cdot2} - p_{x'1\cdot2},$$
$$3 - p_{x0\cdot1} - 2p_{x'0\cdot0} - p_{x'0\cdot1} - 2p_{x1\cdot0} - p_{x1\cdot2} - p_{x'1\cdot2},$$
$$3 - p_{x0\cdot0} - p_{x'0\cdot0} - 2p_{x'0\cdot1} - 2p_{x1\cdot1} - p_{x1\cdot2} - p_{x'1\cdot2},$$
$$2 - p_{x'0\cdot0} - p_{x'0\cdot1} - p_{x1\cdot1} - p_{x1\cdot2} - p_{x'1\cdot2},$$
$$2 - p_{x0\cdot0} - p_{x'0\cdot0} - p_{x'0\cdot1} - p_{x1\cdot1} - p_{x1\cdot2},$$
$$1 + p_{x0\cdot1} - p_{x'0\cdot0} - p_{x''0\cdot0} + p_{x''0\cdot1} + p_{x1\cdot1} - p_{x1\cdot2} + p_{x'1\cdot1},$$

$1 + p_{x0\cdot 2} - p_{x'0\cdot 0} - p_{x''0\cdot 0} + p_{x''0\cdot 1} + p_{x''0\cdot 2} + p_{x1\cdot 1} - p_{x1\cdot 2} + p_{x'1\cdot 1} + p_{x'1\cdot 2},$
$2 - p_{x0\cdot 0} + p_{x0\cdot 1} - p_{x'0\cdot 0} - p_{x'0\cdot 2} - p_{x''0\cdot 0} + p_{x''0\cdot 1} - p_{x''0\cdot 2} + p_{x1\cdot 1} - 2p_{x1\cdot 2} + p_{x'1\cdot 1},$
$2 - p_{x0\cdot 0} - p_{x'0\cdot 0} - p_{x'0\cdot 2} - p_{x''0\cdot 0} + p_{x''0\cdot 1} + p_{x1\cdot 1} - 2p_{x1\cdot 2} + p_{x'1\cdot 1},$
$2 + 2p_{x0\cdot 1} - 2p_{x'0\cdot 0} - 2p_{x''0\cdot 0} + 2p_{x''0\cdot 1} - p_{x1\cdot 0} + p_{x1\cdot 1} - p_{x1\cdot 2} + 2p_{x'1\cdot 1} - p_{x'1\cdot 2},$
$2 + p_{x0\cdot 0} - p_{x0\cdot 1} - p_{x'0\cdot 1} - p_{x'0\cdot 2} + p_{x''0\cdot 0} - p_{x''0\cdot 2} - 2p_{x1\cdot 2} + p_{x'1\cdot 0},$
$2 + p_{x0\cdot 0} - 2p_{x'0\cdot 1} + p_{x''0\cdot 0} - p_{x''0\cdot 1} - p_{x1\cdot 1} - p_{x1\cdot 2} + p_{x'1\cdot 0} - p_{x'1\cdot 2},$
$2 - 2p_{x'0\cdot 1} - p_{x1\cdot 1} - p_{x1\cdot 2} - p_{x'1\cdot 2},$
$2 - p_{x0\cdot 1} - p_{x'0\cdot 1} - p_{x'0\cdot 2} - 2p_{x1\cdot 2},$
$1 - p_{x'0\cdot 1} - p_{x1\cdot 2},$
$2 + p_{x0\cdot 1} - p_{x'0\cdot 0} - p_{x'0\cdot 1} - p_{x''0\cdot 0} + p_{x''0\cdot 1} - p_{x1\cdot 0} - p_{x1\cdot 2} + p_{x'1\cdot 1} - p_{x'1\cdot 2},$
$2 - p_{x0\cdot 1} + p_{x0\cdot 2} - p_{x'0\cdot 0} - p_{x'0\cdot 1} - p_{x''0\cdot 0} + p_{x''0\cdot 2} - p_{x1\cdot 0} - p_{x1\cdot 2} + p_{x'1\cdot 2},$
$2 - p_{x0\cdot 0} + p_{x0\cdot 1} - p_{x'0\cdot 0} - p_{x'0\cdot 2} + p_{x''0\cdot 1} - p_{x''0\cdot 2} - 2p_{x1\cdot 2} + p_{x'1\cdot 1},$
$2 + p_{x0\cdot 1} - 2p_{x'0\cdot 0} - p_{x''0\cdot 0} + p_{x''0\cdot 1} - p_{x1\cdot 0} - p_{x1\cdot 2} + p_{x'1\cdot 1} - p_{x'1\cdot 2},$
$2 - 2p_{x'0\cdot 0} - p_{x1\cdot 0} - p_{x1\cdot 2} - p_{x'1\cdot 2},$
$2 - p_{x0\cdot 0} - p_{x'0\cdot 0} - p_{x'0\cdot 2} - 2p_{x1\cdot 2},$
$1 - p_{x'0\cdot 0} - p_{x1\cdot 2},$
$2 + p_{x0\cdot 0} - p_{x'0\cdot 0} - p_{x'0\cdot 1} + p_{x''0\cdot 0} - p_{x''0\cdot 1} - p_{x1\cdot 1} - p_{x1\cdot 2} + p_{x'1\cdot 0} - p_{x'1\cdot 2},$
$2 - p_{x0\cdot 0} + p_{x0\cdot 2} - p_{x'0\cdot 0} - p_{x'0\cdot 1} - p_{x''0\cdot 1} + p_{x''0\cdot 2} - p_{x1\cdot 1} - p_{x1\cdot 2} + p_{x'1\cdot 2},$
$2 + 2p_{x0\cdot 0} - 2p_{x'0\cdot 1} + 2p_{x''0\cdot 0} - 2p_{x''0\cdot 1} + p_{x1\cdot 0} - p_{x1\cdot 1} - p_{x1\cdot 2} + 2p_{x'1\cdot 0} - p_{x'1\cdot 2},$
$2 - p_{x0\cdot 1} - p_{x'0\cdot 1} - p_{x'0\cdot 2} + p_{x''0\cdot 0} - p_{x''0\cdot 1} + p_{x1\cdot 0} - 2p_{x1\cdot 2} + p_{x'1\cdot 0},$
$1 + p_{x0\cdot 0} - p_{x'0\cdot 1} + p_{x''0\cdot 0} - p_{x''0\cdot 1} + p_{x1\cdot 0} - p_{x1\cdot 2} + p_{x'1\cdot 0},$
$2 + p_{x0\cdot 0} - p_{x0\cdot 1} - p_{x'0\cdot 1} - p_{x'0\cdot 2} + p_{x''0\cdot 0} - p_{x''0\cdot 1} - p_{x''0\cdot 2} + p_{x1\cdot 0} - 2p_{x1\cdot 2} + p_{x'1\cdot 0},$
$1 + p_{x0\cdot 2} - p_{x'0\cdot 1} + p_{x''0\cdot 0} - p_{x''0\cdot 1} + p_{x''0\cdot 2} + p_{x1\cdot 0} - p_{x1\cdot 2} + p_{x'1\cdot 0} + p_{x'1\cdot 2}\}$

# S2 Proof of Results

**Proof Result 1**:

First we derive the bounds for $\theta_{x'x}$ under the following NPSEM:

$$\begin{aligned} z &= g_Z(\epsilon_z) \\ x &= g_X(\boldsymbol{u}, z, \epsilon_x) \\ y &= \begin{cases} g_Y(\boldsymbol{u}, x, \epsilon_y) \text{ if } x \in \{x, x'\} \\ \text{undefined if } x = x^m \end{cases} . \end{aligned} \quad (1)$$

The bounds are similarly derived in Balke [1995], starting on page 118. Since $Z, X$ and $Y$ are all discrete, we can apply the canonical partitioning step of Theorem 1 of Sachs et al. [2023] that yields the following structural equations in terms of discrete response function

variables $r_Z, r_X, r_Y$

$$g_Z(r_Z) = \begin{cases} 0 \text{ if } r_Z = 0 \\ 1 \text{ if } r_Z = 1 \end{cases} .$$

For $X$, the response function variable $r_X$ can take on values $0, 1, \ldots, 8$, and the outputs of the response function $g_X(r_X, Z)$ are defined in the following table:

| $r_X$ | $Z = 0$ | $Z = 1$ |
|---|---|---|
| 0 | $x$ | $x$ |
| 1 | $x'$ | $x$ |
| 2 | $x^m$ | $x$ |
| 3 | $x$ | $x'$ |
| 4 | $x'$ | $x'$ |
| 5 | $x^m$ | $x'$ |
| 6 | $x$ | $x^m$ |
| 7 | $x'$ | $x^m$ |
| 8 | $x^m$ | $x^m$ |

For $Y$, the response function variable $r_Y$ can take on values $0, 1, 2, 3$, with outputs of $g_Y(r_X, X)$ given by

| $r_Y$ | $X = x$ | $X = x'$ | $X = x^m$ |
|---|---|---|---|
| 0 | 0 | 0 | undefined |
| 1 | 1 | 0 | undefined |
| 2 | 0 | 1 | undefined |
| 3 | 1 | 1 | undefined |

Let $q_{i \cdot j} = p(r_X = i, r_Y = j)$ for $i \in \{0, 1, \ldots, 8\}, j \in \{0, 1, 2, 3\}$. Based on the response functions we find constraints in terms of observable conditional probabilities by the relations:

$$p(X = x, Y = y | Z = z) = \sum_{q \in \mathcal{B}} q, \text{ where } \mathcal{B} = \{q_{i \cdot j} : g_X(i, z) = x \text{ and } g_Y(j, z) = y\}.$$

Define the shorthand notation $p(X = x, Y = y | Z = z) = p_{xy \cdot z}$. Then in addition to the natural constraint on probabilities in the first row below, we have

$$\sum_{x \in \{0, \ldots, 8\}} \sum_{y \in \{0,1,2,3\}} q_{x \cdot y} = 1$$

$$p_{x0 \cdot 0} = q_{0 \cdot 0} + q_{0 \cdot 2} + q_{3 \cdot 0} + q_{3 \cdot 2} + q_{6 \cdot 0} + q_{6 \cdot 2}$$

$$p_{x0 \cdot 1} = q_{0 \cdot 0} + q_{0 \cdot 2} + q_{1 \cdot 0} + q_{1 \cdot 2} + q_{2 \cdot 0} + q_{2 \cdot 2}$$

$$p_{x'0 \cdot 0} = q_{1 \cdot 0} + q_{1 \cdot 1} + q_{4 \cdot 0} + q_{4 \cdot 1} + q_{7 \cdot 0} + q_{7 \cdot 1}$$

$$p_{x'0 \cdot 1} = q_{3 \cdot 0} + q_{3 \cdot 1} + q_{4 \cdot 0} + q_{4 \cdot 1} + q_{5 \cdot 0} + q_{5 \cdot 1}$$

$$p_{x1 \cdot 0} = q_{0 \cdot 1} + q_{0 \cdot 3} + q_{3 \cdot 1} + q_{3 \cdot 3} + q_{6 \cdot 1} + q_{6 \cdot 3}$$

$$p_{x1\cdot 1} = q_{0\cdot 1} + q_{0\cdot 3} + q_{1\cdot 1} + q_{1\cdot 3} + q_{2\cdot 1} + q_{2\cdot 3}$$
$$p_{x'1\cdot 0} = q_{1\cdot 2} + q_{1\cdot 3} + q_{4\cdot 2} + q_{4\cdot 3} + q_{7\cdot 2} + q_{7\cdot 3}$$
$$p_{x'1\cdot 1} = q_{3\cdot 2} + q_{3\cdot 3} + q_{4\cdot 2} + q_{4\cdot 3} + q_{5\cdot 2} + q_{5\cdot 3}$$
$$p_{x^m\cdot 0} = q_{2\cdot 0} + q_{2\cdot 1} + q_{2\cdot 2} + q_{2\cdot 3} + q_{5\cdot 0} + q_{5\cdot 1} + q_{5\cdot 2} + q_{5\cdot 3} + q_{8\cdot 0} + q_{8\cdot 1} + q_{8\cdot 2} + q_{8\cdot 3}$$
$$p_{x^m\cdot 1} = q_{6\cdot 0} + q_{6\cdot 1} + q_{6\cdot 2} + q_{6\cdot 3} + q_{7\cdot 0} + q_{7\cdot 1} + q_{7\cdot 2} + q_{7\cdot 3} + q_{8\cdot 0} + q_{8\cdot 1} + q_{8\cdot 2} + q_{8\cdot 3}$$

Using similar relations, but under the modified response function for $X$ with the intervention: $g^*_X(r_X, Z) = x'$ for the first term of the risk difference and $g^*_X(r_X, Z) = x$ for the second term, we can express the risk difference $\theta_{x'x}$ in terms of the $q_{x\cdot y}$ parameters as

$$\theta_{x'x} = \sum_{x=0}^{8} q_{x\cdot 2} - \sum_{x=0}^{8} q_{x\cdot 1}.$$

This is a linear program and thus we can apply a vertex enumeration algorithm to its dual (e.g., the double description method [Motzkin et al., 1953]) to find the bounds as reported in the main text.

After applying the canonical partitioning to the following NPSEM,

$$\begin{aligned} z &= g_Z(\epsilon_z) \\ x^* &= g_X(\boldsymbol{u}, z, \epsilon_{x^*}) \\ x &= g_X(x^*) \\ y &= \begin{cases} f_Y(\boldsymbol{u}, x, \epsilon_y) \text{ if } x \in \{x, x'\} \\ f_Y(\boldsymbol{u}, x, z, \epsilon_y) \text{ if } x = x^m \end{cases} \end{aligned}$$

we get identical response functions for $Z$ and $X$ as above. For $Y$, our $r_Y$ variable can now take on values $0, 1, \ldots, 15$. The outputs of the response function $f_Y(r_Y, z, x)$ is defined in Table S1. Observe that the outputs of $f_Y$ only depend on the value of $Z$ when $X = x^m$, i.e., columns 1, 2 are the same as columns 4, 5, respectively, while columns 3 and 6 differ.

Let $q_{i\cdot j} = p(r_X = i, r_Y = j)$ and $k_z = p(r_Z = z)$. Observe that $r_Z$ is independent of $r_X$ and $r_Y$. This causal model does fit into the class with linear constraints as defined by Theorem 2 of Sachs et al. [2023]. This set of response functions yields the following linear constraints on the observable probabilities:

$$\sum_{i\in\{0,\ldots,8\}} \sum_{j\in\{0,1,2,3\}} q_{i\cdot j} = 1$$
$$\begin{aligned} p_{x0\cdot 0} = {} & q_{0\cdot 0} + q_{0\cdot 1} + q_{0\cdot 12} + q_{0\cdot 13} + q_{0\cdot 4} + q_{0\cdot 5} + q_{0\cdot 8} + q_{0\cdot 9} + q_{3\cdot 0} + q_{3\cdot 1} + q_{3\cdot 12} + q_{3\cdot 13} + q_{3\cdot 4} \\ & + q_{3\cdot 5} + q_{3\cdot 8} + q_{3\cdot 9} + q_{6\cdot 0} + q_{6\cdot 1} + q_{6\cdot 12} + q_{6\cdot 13} + q_{6\cdot 4} + q_{6\cdot 5} + q_{6\cdot 8} + q_{6\cdot 9} \end{aligned}$$
$$\begin{aligned} p_{x0\cdot 1} = {} & q_{0\cdot 0} + q_{0\cdot 1} + q_{0\cdot 12} + q_{0\cdot 13} + q_{0\cdot 4} + q_{0\cdot 5} + q_{0\cdot 8} + q_{0\cdot 9} + q_{1\cdot 0} + q_{1\cdot 1} + q_{1\cdot 12} + q_{1\cdot 13} + q_{1\cdot 4} \\ & + q_{1\cdot 5} + q_{1\cdot 8} + q_{1\cdot 9} + q_{2\cdot 0} + q_{2\cdot 1} + q_{2\cdot 12} + q_{2\cdot 13} + q_{2\cdot 4} + q_{2\cdot 5} + q_{2\cdot 8} + q_{2\cdot 9} \end{aligned}$$
$$\begin{aligned} p_{x'0\cdot 0} = {} & q_{1\cdot 0} + q_{1\cdot 1} + q_{1\cdot 10} + q_{1\cdot 11} + q_{1\cdot 2} + q_{1\cdot 3} + q_{1\cdot 8} + q_{1\cdot 9} + q_{4\cdot 0} + q_{4\cdot 1} + q_{4\cdot 10} + q_{4\cdot 11} + q_{4\cdot 2} \\ & + q_{4\cdot 3} + q_{4\cdot 8} + q_{4\cdot 9} + q_{7\cdot 0} + q_{7\cdot 1} + q_{7\cdot 10} + q_{7\cdot 11} + q_{7\cdot 2} + q_{7\cdot 3} + q_{7\cdot 8} + q_{7\cdot 9} \end{aligned}$$

| | $(X, Z)$ | | | | | |
|---|---|---|---|---|---|---|
| $r_Y$ | $(x, 0)$ | $(x', 0)$ | $(x^m, 0)$ | $(x, 1)$ | $(x', 1)$ | $(x^m, 1)$ |
| 0 | 0 | 0 | 0 | 0 | 0 | 0 |
| 1 | 0 | 0 | 1 | 0 | 0 | 0 |
| 2 | 1 | 0 | 0 | 1 | 0 | 0 |
| 3 | 1 | 0 | 1 | 1 | 0 | 0 |
| 4 | 0 | 1 | 0 | 0 | 1 | 0 |
| 5 | 0 | 1 | 1 | 0 | 1 | 0 |
| 6 | 1 | 1 | 0 | 1 | 1 | 0 |
| 7 | 1 | 1 | 1 | 1 | 1 | 0 |
| 8 | 0 | 0 | 0 | 0 | 0 | 1 |
| 9 | 0 | 0 | 1 | 0 | 0 | 1 |
| 10 | 1 | 0 | 0 | 1 | 0 | 1 |
| 11 | 1 | 0 | 1 | 1 | 0 | 1 |
| 12 | 0 | 1 | 0 | 0 | 1 | 1 |
| 13 | 0 | 1 | 1 | 0 | 1 | 1 |
| 14 | 1 | 1 | 0 | 1 | 1 | 1 |
| 15 | 1 | 1 | 1 | 1 | 1 | 1 |

Table S1: Response function for $Y$ in the partially contaminated IV setting.

$$
\begin{aligned}
p_{x'0\cdot 1} &= q_{3\cdot 0} + q_{3\cdot 1} + q_{3\cdot 10} + q_{3\cdot 11} + q_{3\cdot 2} + q_{3\cdot 3} + q_{3\cdot 8} + q_{3\cdot 9} + q_{4\cdot 0} + q_{4\cdot 1} + q_{4\cdot 10} + q_{4\cdot 11} + q_{4\cdot 2} \\
&\quad + q_{4\cdot 3} + q_{4\cdot 8} + q_{4\cdot 9} + q_{5\cdot 0} + q_{5\cdot 1} + q_{5\cdot 10} + q_{5\cdot 11} + q_{5\cdot 2} + q_{5\cdot 3} + q_{5\cdot 8} + q_{5\cdot 9} \\
p_{x^m0\cdot 0} &= q_{2\cdot 0} + q_{2\cdot 10} + q_{2\cdot 12} + q_{2\cdot 14} + q_{2\cdot 2} + q_{2\cdot 4} + q_{2\cdot 6} + q_{2\cdot 8} + q_{5\cdot 0} + q_{5\cdot 10} + q_{5\cdot 12} + q_{5\cdot 14} + q_{5\cdot 2} \\
&\quad + q_{5\cdot 4} + q_{5\cdot 6} + q_{5\cdot 8} + q_{8\cdot 0} + q_{8\cdot 10} + q_{8\cdot 12} + q_{8\cdot 14} + q_{8\cdot 2} + q_{8\cdot 4} + q_{8\cdot 6} + q_{8\cdot 8} \\
p_{x^m0\cdot 1} &= q_{6\cdot 0} + q_{6\cdot 1} + q_{6\cdot 2} + q_{6\cdot 3} + q_{6\cdot 4} + q_{6\cdot 5} + q_{6\cdot 6} + q_{6\cdot 7} + q_{7\cdot 0} + q_{7\cdot 1} + q_{7\cdot 2} + q_{7\cdot 3} + q_{7\cdot 4} + q_{7\cdot 5} \\
&\quad + q_{7\cdot 6} + q_{7\cdot 7} + q_{8\cdot 0} + q_{8\cdot 1} + q_{8\cdot 2} + q_{8\cdot 3} + q_{8\cdot 4} + q_{8\cdot 5} + q_{8\cdot 6} + q_{8\cdot 7} \\
p_{x1\cdot 0} &= q_{0\cdot 10} + q_{0\cdot 11} + q_{0\cdot 14} + q_{0\cdot 15} + q_{0\cdot 2} + q_{0\cdot 3} + q_{0\cdot 6} + q_{0\cdot 7} + q_{3\cdot 10} + q_{3\cdot 11} + q_{3\cdot 14} + q_{3\cdot 15} + q_{3\cdot 2} \\
&\quad + q_{3\cdot 3} + q_{3\cdot 6} + q_{3\cdot 7} + q_{6\cdot 10} + q_{6\cdot 11} + q_{6\cdot 14} + q_{6\cdot 15} + q_{6\cdot 2} + q_{6\cdot 3} + q_{6\cdot 6} + q_{6\cdot 7} \\
p_{x1\cdot 1} &= q_{0\cdot 10} + q_{0\cdot 11} + q_{0\cdot 14} + q_{0\cdot 15} + q_{0\cdot 2} + q_{0\cdot 3} + q_{0\cdot 6} + q_{0\cdot 7} + q_{1\cdot 10} + q_{1\cdot 11} + q_{1\cdot 14} + q_{1\cdot 15} + q_{1\cdot 2} \\
&\quad + q_{1\cdot 3} + q_{1\cdot 6} + q_{1\cdot 7} + q_{2\cdot 10} + q_{2\cdot 11} + q_{2\cdot 14} + q_{2\cdot 15} + q_{2\cdot 2} + q_{2\cdot 3} + q_{2\cdot 6} + q_{2\cdot 7} \\
p_{x'1\cdot 0} &= q_{1\cdot 12} + q_{1\cdot 13} + q_{1\cdot 14} + q_{1\cdot 15} + q_{1\cdot 4} + q_{1\cdot 5} + q_{1\cdot 6} + q_{1\cdot 7} + q_{4\cdot 12} + q_{4\cdot 13} + q_{4\cdot 14} + q_{4\cdot 15} + q_{4\cdot 4} \\
&\quad + q_{4\cdot 5} + q_{4\cdot 6} + q_{4\cdot 7} + q_{7\cdot 12} + q_{7\cdot 13} + q_{7\cdot 14} + q_{7\cdot 15} + q_{7\cdot 4} + q_{7\cdot 5} + q_{7\cdot 6} + q_{7\cdot 7} \\
p_{x'1\cdot 1} &= q_{3\cdot 12} + q_{3\cdot 13} + q_{3\cdot 14} + q_{3\cdot 15} + q_{3\cdot 4} + q_{3\cdot 5} + q_{3\cdot 6} + q_{3\cdot 7} + q_{4\cdot 12} + q_{4\cdot 13} + q_{4\cdot 14} + q_{4\cdot 15} + q_{4\cdot 4} \\
&\quad + q_{4\cdot 5} + q_{4\cdot 6} + q_{4\cdot 7} + q_{5\cdot 12} + q_{5\cdot 13} + q_{5\cdot 14} + q_{5\cdot 15} + q_{5\cdot 4} + q_{5\cdot 5} + q_{5\cdot 6} + q_{5\cdot 7} \\
p_{x^m1\cdot 0} &= q_{2\cdot 1} + q_{2\cdot 11} + q_{2\cdot 13} + q_{2\cdot 15} + q_{2\cdot 3} + q_{2\cdot 5} + q_{2\cdot 7} + q_{2\cdot 9} + q_{5\cdot 1} + q_{5\cdot 11} + q_{5\cdot 13} + q_{5\cdot 15} + q_{5\cdot 3} \\
&\quad + q_{5\cdot 5} + q_{5\cdot 7} + q_{5\cdot 9} + q_{8\cdot 1} + q_{8\cdot 11} + q_{8\cdot 13} + q_{8\cdot 15} + q_{8\cdot 3} + q_{8\cdot 5} + q_{8\cdot 7} + q_{8\cdot 9} \\
p_{x^m1\cdot 1} &= q_{6\cdot 10} + q_{6\cdot 11} + q_{6\cdot 12} + q_{6\cdot 13} + q_{6\cdot 14} + q_{6\cdot 15} + q_{6\cdot 8} + q_{6\cdot 9} + q_{7\cdot 10} + q_{7\cdot 11} + q_{7\cdot 12} + q_{7\cdot 13} \\
&\quad + q_{7\cdot 14} + q_{7\cdot 15} + q_{7\cdot 8} + q_{7\cdot 9} + q_{8\cdot 10} + q_{8\cdot 11} + q_{8\cdot 12} + q_{8\cdot 13} + q_{8\cdot 14} + q_{8\cdot 15} + q_{8\cdot 8} + q_{8\cdot 9}
\end{aligned}
$$

Due to the dependence of $f_Y$ on $Z$, the $\theta_{x'x}$ does not fit into the class of effects that

are guaranteed to be linear according to Theorem 3 of Sachs et al. [2023]. In particular, we must consider the response function variables $k_0, k_0$ in addition to the $q$s. Consider the first term $p(Y(X = x') = 1)$. Under the modified $g^*_X(r_X, Z) = x'$, and with $\mathcal{B} = \{i, j, d : f_Y(r_j, g^*_X(r_i, g_Z(r_d)), g_Z(r_d)) = 1\}$ we have

$$\sum_{\mathcal{B}} p(r_Z = d)p(r_X = i, r_Y = j) =$$

$$k_0q_{0\cdot12} + k_1q_{0\cdot12} + k_1q_{0\cdot13} + k_0q_{0\cdot13} + k_0q_{0\cdot14} + k_1q_{0\cdot14} + k_0q_{0\cdot15} + k_1q_{0\cdot15} + k_0q_{0\cdot4} + k_1q_{0\cdot4} + k_0q_{0\cdot5}$$
$$+ k_1q_{0\cdot5} + k_0q_{0\cdot6} + k_1q_{0\cdot6} + k_0q_{0\cdot7} + k_1q_{0\cdot7} + k_1q_{1\cdot12} + k_0q_{1\cdot12} + k_1q_{1\cdot13} + k_0q_{1\cdot13} + k_1q_{1\cdot14}$$
$$+ k_0q_{1\cdot14} + k_1q_{1\cdot15} + k_0q_{1\cdot15} + k_1q_{1\cdot4} + k_0q_{1\cdot4} + k_0q_{1\cdot5} + k_1q_{1\cdot5} + k_0q_{1\cdot6} + k_1q_{1\cdot6} + k_1q_{1\cdot7}$$
$$+ k_0q_{1\cdot7} + k_1q_{2\cdot12} + k_0q_{2\cdot12} + k_1q_{2\cdot13} + k_0q_{2\cdot13} + k_0q_{2\cdot14} + k_1q_{2\cdot14} + k_0q_{2\cdot15} + k_1q_{2\cdot15} + k_1q_{2\cdot4}$$
$$+ k_0q_{2\cdot4} + k_1q_{2\cdot5} + k_0q_{2\cdot5} + k_1q_{2\cdot6} + k_0q_{2\cdot6} + k_1q_{2\cdot7} + k_0q_{2\cdot7} + k_0q_{3\cdot12} + k_1q_{3\cdot12} + k_0q_{3\cdot13}$$
$$+ k_1q_{3\cdot13} + k_0q_{3\cdot14} + k_1q_{3\cdot14} + k_0q_{3\cdot15} + k_1q_{3\cdot15} + k_1q_{3\cdot4} + k_0q_{3\cdot4} + k_0q_{3\cdot5} + k_1q_{3\cdot5} + k_0q_{3\cdot6}$$
$$+ k_1q_{3\cdot6} + k_1q_{3\cdot7} + k_0q_{3\cdot7} + k_0q_{4\cdot12} + k_1q_{4\cdot12} + k_0q_{4\cdot13} + k_1q_{4\cdot13} + k_0q_{4\cdot14} + k_1q_{4\cdot14} + k_0q_{4\cdot15}$$
$$+ k_1q_{4\cdot15} + k_0q_{4\cdot4} + k_1q_{4\cdot4} + k_0q_{4\cdot5} + k_1q_{4\cdot5} + k_0q_{4\cdot6} + k_1q_{4\cdot6} + k_0q_{4\cdot7} + k_1q_{4\cdot7} + k_1q_{5\cdot12}$$
$$+ k_0q_{5\cdot12} + k_0q_{5\cdot13} + k_1q_{5\cdot13} + k_1q_{5\cdot14} + k_0q_{5\cdot14} + k_1q_{5\cdot15} + k_0q_{5\cdot15} + k_0q_{5\cdot4} + k_1q_{5\cdot4} + k_0q_{5\cdot5}$$
$$+ k_1q_{5\cdot5} + k_0q_{5\cdot6} + k_1q_{5\cdot6} + k_0q_{5\cdot7} + k_1q_{5\cdot7} + k_1q_{6\cdot12} + k_0q_{6\cdot12} + k_1q_{6\cdot13} + k_0q_{6\cdot13} + k_1q_{6\cdot14}$$
$$+ k_0q_{6\cdot14} + k_0q_{6\cdot15} + k_1q_{6\cdot15} + k_0q_{6\cdot4} + k_1q_{6\cdot4} + k_1q_{6\cdot5} + k_0q_{6\cdot5} + k_1q_{6\cdot6} + k_0q_{6\cdot6} + k_1q_{6\cdot7}$$
$$+ k_0q_{6\cdot7} + k_0q_{7\cdot12} + k_1q_{7\cdot12} + k_0q_{7\cdot13} + k_1q_{7\cdot13} + k_0q_{7\cdot14} + k_1q_{7\cdot14} + k_0q_{7\cdot15} + k_1q_{7\cdot15} + k_1q_{7\cdot4}$$
$$+ k_0q_{7\cdot4} + k_1q_{7\cdot5} + k_0q_{7\cdot5} + k_0q_{7\cdot6} + k_1q_{7\cdot6} + k_1q_{7\cdot7} + k_0q_{7\cdot7} + k_0q_{8\cdot12} + k_1q_{8\cdot12} + k_0q_{8\cdot13}$$
$$+ k_1q_{8\cdot13} + k_0q_{8\cdot14} + k_1q_{8\cdot14} + k_0q_{8\cdot15} + k_1q_{8\cdot15} + k_0q_{8\cdot4} + k_1q_{8\cdot4} + k_0q_{8\cdot5} + k_1q_{8\cdot5} + k_0q_{8\cdot6}$$
$$+ k_1q_{8\cdot6} + k_0q_{8\cdot7} + k_1q_{8\cdot7}$$

Observe that for every $q_{x\cdot y}$ term that appears in this equation, we have the sum

$$k_0q_{x\cdot y} + k_1q_{x\cdot y} = p(r_Z = 0)p(r_X = x, r_Y = y) + p(r_Z = 1)p(r_X = x, r_Y = y) = q_{x\cdot y},$$

i.e., the response function variables $k_z$ get marginalized out. This also occurs for the second term of the risk difference $p(Y(X = x) = 1)$, and we then have a linear objective function that is only in terms of the $q$ probabilities. Then we apply the vertex enumeration method and obtain the bounds. This marginalization of the $k_z$ occurs because the contrast does not involve the level $x^m$; any contrast or probability that does involve $x^m$ leads to a nonlinear objective function.

Visual inspection of the terms of the bounds allows us to verify that they are the same as those derived above under the setting of two well-defining levels and third ill-defining level. Further inspection and comparison to the standard binary IV bounds allows us to verify that they are also the same expressions, proving Result 1.

**Proof Result 2**:

In this case with one well-defining level of $X$, $x$ and one potentially ill-defining level $x^m$,

we have the response function for $Z$

$$g_Z(r_Z) = \begin{cases} 0 \text{ if } r_Z = 0 \\ 1 \text{ if } r_Z = 1 \end{cases}$$

The response function for $X$ is defined in the following table.

| $r_X$ | $Z = 0$ | $Z = 1$ |
|---|---|---|
| 0 | $x$ | $x$ |
| 1 | $x^m$ | $x$ |
| 2 | $x$ | $x^m$ |
| 3 | $x^m$ | $x^m$ |

For $Y$, the response function variable $r_Y$ can take on values $0, 1$, with outputs of $f_Y(r_Y, X)$ given by

| $r_Y$ | $X = x$ | $X = x^m$ |
|---|---|---|
| 0 | 0 | undefined |
| 1 | 1 | undefined |

We follow the same steps as above with these response functions to find the linear program, which we then solve by vertex enumeration. The resulting bounds are as reported in the main text.

In the case where there are two well-defining levels given one of which, $x^m$, the IV has a direct effect on the outcome, we have the same response functions for $X$ and $Z$, but the response function for $Y$, $f_Y(r_Y, X, Z)$ is defined in the following table:

| | $(X, Z)$ | | | |
|---|---|---|---|---|
| $r_Y$ | $(x, 0)$ | $(x^m, 0)$ | $(x, 1)$ | $(x^m, 1)$ |
| 0 | 0 | 0 | 0 | 0 |
| 1 | 0 | 1 | 0 | 0 |
| 2 | 1 | 0 | 1 | 0 |
| 3 | 1 | 1 | 1 | 0 |
| 4 | 0 | 0 | 0 | 1 |
| 5 | 0 | 1 | 0 | 1 |
| 6 | 1 | 0 | 1 | 1 |
| 7 | 1 | 1 | 1 | 1 |

Again, the constraints on the observable probabilities are linear because this fits into the class of defined in Theorem 2 of Sachs et al. [2023]. Since the output of the response function for $Y$ does not depend on $Z$ when $X = x$, just as above, we are able to marginalize out the probabilities of $r_Z$ when deriving the objective function in terms of the response function variable probabilities. Thus we again have a linear program which we can solve using vertex enumeration, and the result yields the bounds as reported in the main text, proving Result 2.

**Proof of Results 3 and 4**:

Results 3 and 4 can be proven in a similar manner as Result 1. Due to the three-level IV, the response functions have more outputs compared to result 1, but the steps of the proof can be followed in the same way to show that although the cases do not fall into the class of problems known to be linear according to Sachs et al. [2023], they are in fact linear programs that can be solved by vertex enumeration.

# References


A. Balke and J. Pearl. Bounds on treatment effects from studies with imperfect compliance. *Journal of the American Statistical Association*, 92:1171–1176, 1997.

Alexander A Balke. *Probabilistic Counterfactuals: Semantics, Computation, and Applications*. PhD thesis, Department of Computer Science, University of California, Los Angeles, 1995.

T.S. Motzkin, H. Raiffa, GL. Thompson, and R.M. Thrall. The double description method. *Contributions to Theory of Games*, 2, 1953.

Michael C Sachs, Gustav Jonzon, Arvid Sjölander, and Erin E Gabriel. A general method for deriving tight symbolic bounds on causal effects. *Journal of Computational and Graphical Statistics*, 32(2):567–576, 2023.
